# Supplementary material for: Limits of economy and fidelity for programmable assembly of size-controlled triply-periodic polyhedra
Source: arXiv:2309.04632 ancillary file (2023-09-08)
Supplement: Supplementary file 1 [file SI.pdf]

# Supporting Information: Limits of economy and fidelity for programmable assembly of size-controlled triply-periodic polyhedra

Carlos M. Duque,<sup>1,2,3</sup> Douglas M. Hall,<sup>4</sup> Botond Tyukodi,<sup>5</sup> Michael F. Hagan,<sup>6</sup> Christian D. Santangelo,<sup>6</sup> and Gregory M. Grason<sup>4</sup>

<sup>1</sup>*Max Planck Institute of Molecular Cell Biology and Genetics, 01307 Dresden, Germany*

<sup>2</sup>*Center for Systems Biology Dresden (CSBD), 01307 Dresden, Germany*

<sup>3</sup>*Department of Physics, University of Massachusetts, Amherst, MA 01003*

<sup>4</sup>*Department of Polymer Science and Engineering,  
University of Massachusetts, Amherst, MA 01003*

<sup>5</sup>*Department of Physics, Babes-Bolyai University, 400084 Cluj-Napoca, Romania*

<sup>6</sup>*Martin A. Fisher School of Physics, Brandeis University, Waltham MA 02453*

## I. EXTENSION OF CASPAR KLUG CONSTRUCTION TO P,G,D TRIANGULATIONS

The construction of Caspar and Klug is a procedure to create structures with increasing number of subunits proportional to the triangulation number  $T$  while preserving icosahedral symmetry [1]. The extension of this construction to the structures studied here was formulated previously [2], considering the dual problem of packing spheres on the surface with packing deriving from hexagonal packing of the plane. Here, we give an explicit procedure for deriving the sub-triangulations ( $T > 1$ ) derived from base triangulations ( $T = 1$ ) of the P,G, and D surfaces based on the principles of Caspar and Klug. In each case, the vertices of the base triangulations are identified with vertices and centers of the hexagonal base tiles associated with each structure.

The steps of the construction are outlined in Fig 11, yielding explicit coordinates for vertices of each triangle in the cubic unit cell. The  $T = 1$  structure is taken as a starting point, which is then sub-divided to the desired triangulation number. Finally, each vertex is translated by gradient flow along an objective function to arrive closer to an approximation of the target surface.

From the  $T = 1$  structure, both the coordinates of each triangle's vertices in the unit cell is known and also an indexing of each triangle's neighbors is derived by identifying which edges are shared by which triangles. The extended construction is to then identify a part of the planar triangular lattice with each triangles of  $T = 1$  by an orthogonal projection: each edge of the  $T = 1$  structure corresponds to a vector  $\mathbf{L} = h\mathbf{a}_1 + k\mathbf{a}_2$  of the planar structure with standard triangular lattice vectors  $\mathbf{a}_1, \mathbf{a}_2$ . The triangulation indices  $h, k$  are integers that enumerate different triangulation numbers via the relation  $T = h^2 + k^2 + hk$  that derives from the area of the equilateral triangle with edge  $\mathbf{L}$  expressed in units of the original triangular lattice vectors' length.

Adjacent edges on the  $T = 1$  structure are identified with vectors in the planar diagram  $\mathbf{L}, \mathbf{U}_1 = -k\mathbf{a}_1 + (h+k)\mathbf{a}_2$  and  $\mathbf{U}_2 = (h+k)\mathbf{a}_1 - h\mathbf{a}_2$ . Each vertex contained in the triangle with edges  $\mathbf{L}, \mathbf{U}_1$  can be expressed as  $i\mathbf{a}_1 + j\mathbf{a}_2$ , and equivalently as  $\frac{1}{T}(i(h+k) + jk)\mathbf{L} + \frac{1}{T}(jh - ik)\mathbf{U}_1$ . This mapping of vertices is an orthographic projection, so that while the triangulation of the icosahedron in this manner will yield equilateral triangles, here isosceles triangles are found due to the isosceles triangles of  $T = 1$  deriving from the asymmetric units of P,G and D. The edges of the ( $T > 1$ ) triangulation follow from the mapping identifying  $\mathbf{L}, \mathbf{U}_1$  and the additional identification of  $\mathbf{U}_2$  wherever an edge of the planar diagram crosses over the vector  $\mathbf{L}$ .

The resulting sub-triangulations are planar except for triangles near the boundary. In the final step to construct the explicit coordinates of the  $T > 1$  triangulation, in the spirit of quasi-equivalence, vertices of the sub-triangulation are each translated by gradient flow along the function  $f^i$  ( $i = P, G, D$ ) to the nodal approximation of the target surface  $f = 0$  while minimizing the distance that each vertex is translated from its initial value. This is performed by using Mathematica software to minimize  $\|\mathbf{x} - \mathbf{x}_0\|^2$  subject to the constraint  $f(\mathbf{x}) = 0$ . While the vertices are transformed, the edge topology is kept the same by preserving the edge data according to indexing of each vertex before and after the gradient flow. This final step preserves the symmetries of the structure because each  $f(x, y, z)$  has the targeted symmetries.

## II. DERIVATION OF MATCHING RULES AND GEOMETRIC PARAMETERS FOR SIMULATION

With the cubic unit cell of structures derived using the construction of the previous section, we next consider the matching rules for building blocks that exactly address the target structure in the rigid limit, of zero compliance in either bending or stretching. We consider the minimal number of subunit types required where each subunit has three edges, each edge has a single length, dihedral angle with respect to its neighbor, and only binds with exactly one

subunit type and a single corresponding edge index (see figure 2). When comparing to triangulations of icosahedral shells and other deltahedral shells, we further allow a triangle to adopt three-fold symmetry, so that each of its three edges have the same lengths, dihedrals, and bind to a single edge identity.

The types and matching rules may be identified in the unit cell directly from the identifications found by applying the discrete symmetries of the corresponding target surface. For the purpose of generating matching rules for the simulations, we only use the translational and rotational symmetries (no inversion or mirror symmetry), resulting in twice the number of subunit species with distinct species that are related by the additional symmetries not considered. Taking advantage of the rotoinversion symmetries of the ultimate triangulations in  $\mathbb{E}^3$  then allows us further to identify “flipped” triangle pairs, as a single sub unit type.

In principle, the explicit construction detailed above in the previous section will preserve these symmetries from the original structure, since we are applying orthogonal projection of a three-fold symmetric structure onto the the  $T = 1$  structure and gradient flow according to a function that has the same symmetry. We have developed a method to check whether the numerical procedure for construction preserves symmetry by re-deriving type and matching rule assignment from a given triangulation with vertex coordinates and indexing of triangle neighbors. The procedure is an exhaustive search of all possible assignments, made simpler by the method of constraint propagation: successive sub-symmetries are found by attempting to identify pairs of triangles and their orientations, and propagating the additional identifications that are necessary for such a structure.

The constraint propagation of an identification follows from recursive evaluations of local matches on the collection of triangles  $\{t_i\}$  of the explicit triangulation of the unit cell. A list of proposed type assignments is maintained, with each  $t_i$  having a type and a rotation relative to other members of the type. Each type has an additional Boolean value assigning three-fold symmetry. At each recursion, a proposed match is  $t_a$  and  $t_b$  and a rotation  $r$  that identifies side  $j$  of  $t_a$  with side  $j + r \bmod 3$  of  $t_b$ . The recursion consists of the following:

1. For all three sides  $j = 1..3$ , check that corresponding side lengths and dihedrals match.
2. If this local match fails, the entire propagation terminates and the type assignment is rejected.
3. If the local match succeeds but has been previously identified, no additional matching is required (this is the base case to the recursion).
4. If the local match succeeds but  $t_a$  and  $t_b$  were previously identified to be the same type but with a different rotation, and furthermore no threefold symmetry was previously identified, then threefold symmetry is proposed for this type. Two recursive calls are made to identify  $j = 1$   $j = 2$  and  $j = 1$   $j = 3$  neighbors of  $t_a$ , with rotations such that the corresponding edges shared with  $t_a$  are identified.
5. If the match succeeds and  $t_a$  and  $t_b$  are different types, then the proposed type assignments is updated to reflect their proposed identification. All triangles of the same type as  $t_b$  are assigned the same type as  $t_a$  and their relative rotations with respect to  $t_a$  follow from the their relation to  $t_b$  and the new proposed rotation  $r$  from  $t_a$  to  $t_b$ . Three recursive calls are made to identify neighbor  $j$  of  $t_a$  with neighbor  $j + r \bmod 3$  of  $t_b$ , with the appropriate rotations that derive from the identifications of the sides of  $t_a$  and  $t_b$ , starting again at step 1 each time.

The result of applying this matching algorithm for all possible pairs and possible rotations is that a minimal number of types is identified. The appropriate side lengths and dihedrals for each type can be found from any triangle that has that type, and the matching rules are found from the types of each neighbor. This algorithm was implemented in Mathematica, which is included as supplementary information.

### III. GROUND STATE ENERGIES OF TOPOLOGICAL DEFECTS AND EFFECT OF EXCLUDER SIZE

In order to show that the overabundance of positive defects cannot be readily attributed to some elastic favorability of positive defects we calculated the ratio  $E(+|s|)/E(-|s|)$ , where  $E(\pm|s|)$  are the ground state elastic energies of defect patches of charge  $\pm|s|$ . We performed energy minimizations as a function of the ratio  $\eta_s/\eta_b \sim k/\kappa$ , with  $k$  and  $\kappa$  being the moduli for stretching and dihedral bending respectively. We considered defect patches for the charges  $s = \pm 2\pi/3$  and  $s = \pm\pi$  for  $G_7$  using the patch topologies shown on Fig. 5A. Each energy minimization was done in Mathematica with a conjugate gradient algorithm and using the geometry of the patches of Fig. 5A as initial conditions. In Fig. 9A we show the ratios for charge magnitudes  $|s| = 2\pi/3$  and  $|s| = \pi$ . In general, we do not observe a regime in which positive defects have a much smaller elastic cost than negative defects. On one hand, positive defects appear to have a higher elastic energy cost than their negative counterparts for  $\eta_s/\eta_b \lesssim 10$ . On the other hand, the positive to negative elastic cost becomes comparable for  $\eta_s/\eta_b \gtrsim 10$ . These results suggest then the necessity of a different mechanism in order to rationalize the excess of positive charges.

In Fig. 9B we investigate how steric interactions are reflected on the overall excess of positive charges for the case of  $G_7$  structures. We probe the defect imbalance by measuring the quantities  $n_+$  and  $n_-$  of a given structure which are defined as the total number of charges of positive and negative sign respectively. Defining  $n_{\text{total}} = n_+ + n_-$  and  $\Delta n = n_+ - n_-$ , we measure the mean relative counts difference between positive and negative charges,  $\langle \Delta n / n_{\text{total}} \rangle$ , and

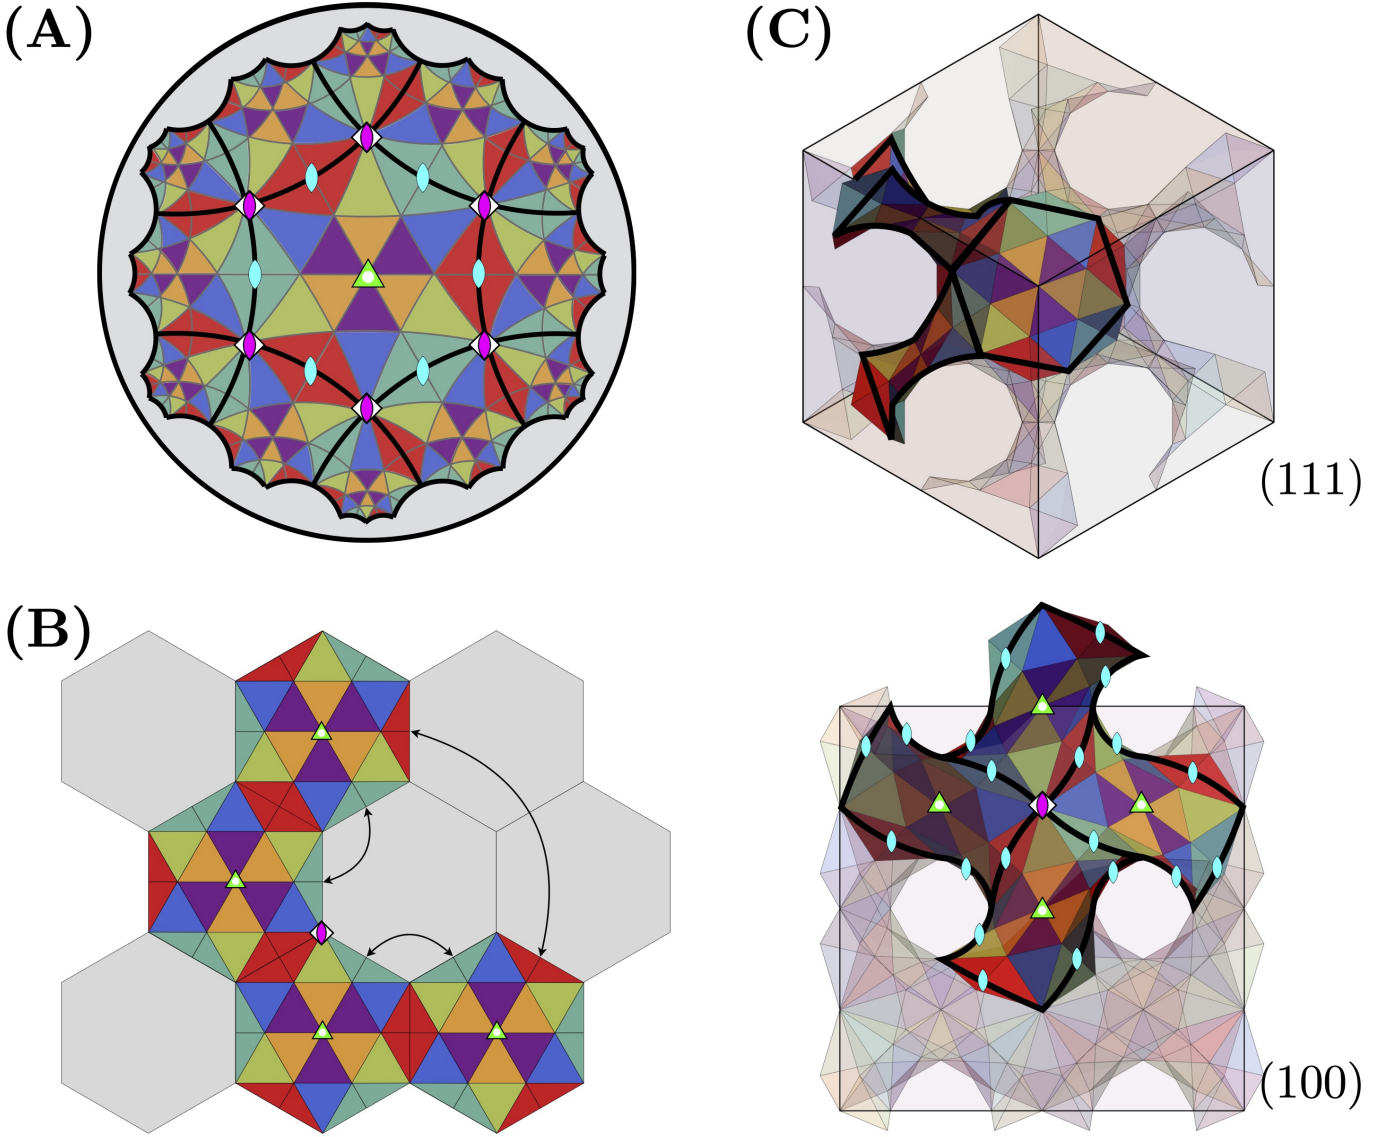

FIG. 1: **(A)**  $T=3$  triangulation projected onto  $\mathbb{H}^2$ . The triangles are colored following the ID labels assigned to triangular subunits of  $T=3$  triply-periodic polyhedra. The thick black lines correspond to the lines of the  $\{6,4\}$  hyperbolic tessellation which can be further subdivided using a single non-Euclidean triangular mono-tile with internal angles  $\{\pi/3, \pi/4, \pi/4\}$  corresponding to the  $T=1$  case. The vertices marked with glyphs are points that map to Wyckoff sites associated to the space groups of the different TPMS. **(B)** Planar template illustrating how the sides of 4 hexagonal  $T=3$  tiles should be identified in order to perform a folding and distorting procedure leading to the  $\mathbb{E}^3$  arrangement shown on **(C)** for the  $G_3$  case in which they all meet at a single vertex of  $\bar{4}$  symmetry.

explore how it varies as the size of the normalized excluder radius between adjacent subunits,  $R_{\text{exc}}/\langle\ell_0\rangle$ , is increased. We fixed the chemical potential,  $\mu = -4.5k_B T$ , and considered three different values for binding affinity between subunits,  $\epsilon_{\text{bind}}$ . To calculate the mean values 10 independent realizations per point were considered. Simulations were run for  $50 \times 10^6$  Monte Carlo steps or until the number of assembled subunits was at least  $N_{\text{total}} = 5000$ . For each  $\epsilon_{\text{bind}}$  we found that as  $R_{\text{exc}}/\langle\ell_0\rangle$  increases,  $\langle\Delta n/n_{\text{total}}\rangle$  tends to saturate to values  $\sim 1$  which we interpret as a clear signature of the fact that negative defects tend to be suppressed as the excluder radius increases. In other words, the allowed configurations of multiple subunits around a given vertex is considerably impacted by the size of the excluder radius of neighboring subunits.

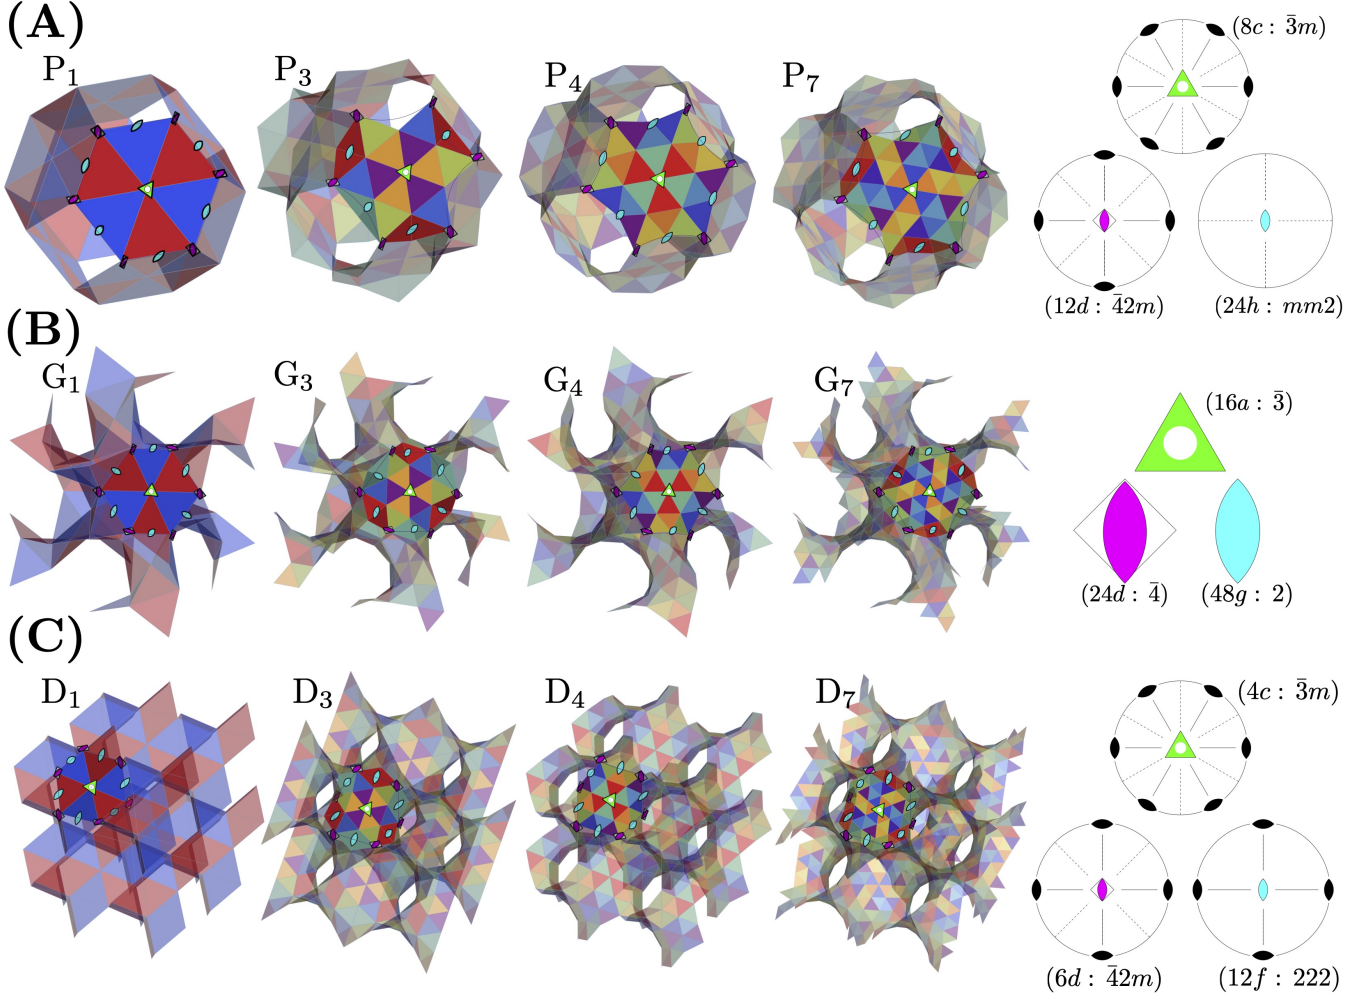

FIG. 2: Wyckoff sites of triply-periodic polyhedral crystals. (A-C) Wyckoff sites of different symmetry are present on the fundamental hexagonal patches of  $P_T$ ,  $G_T$  and  $D_T$  respectively. The symmetry of each Wyckoff site is encoded by one of the glyphs shown on the right panels. Notice that sites with symmetries  $8c$ ,  $16a$ , and  $4c$  as well as  $12d$ ,  $24d$ , and  $6d$  are present for all shown  $T$  numbers of  $P_T$ ,  $G_T$  and  $D_T$  respectively. Among these,  $P_4$ ,  $G_4$ , and  $D_4$  respectively, lead to an addition family of 2-fold symmetric vertices at  $24h$ ,  $48g$ , and  $12f$ .

#### IV. PRECLOSURE BIAS AND ORIGIN OF STRINGY STRUCTURES

In Fig. 9C we further explore the bias for defect preclosure and calculate  $\langle n(s)_{uc} \rangle$ , the mean total number of defects with charge  $s$  per unit-cell and study how  $\langle n(s)_{uc} \rangle$  varies with increasing binding affinity  $\epsilon_{bind}$ . We work again with  $G_7$  and fix the chemical potential and excluder radius to  $\mu = -4.5k_B T$  and  $R_{exc}/\langle \ell_0 \rangle = 0.26$  respectively. Furthermore, we set  $\eta_s = 1$  and  $\eta_b = 0.01$  and solved for the elastic moduli  $k$  and  $\kappa$  by normalizing with respect to the binding affinity value,  $\epsilon_{bind} = -6.5k_B T$ , used throughout the main text. We used the same stopping criteria of the previous section and considered 50 independent Monte Carlo realizations. As  $\epsilon_{bind}/k_B T$  grows large and edge binding moves become more favorable the amounts of positively charged defects, namely  $s = +2\pi/3, +\pi$ , increase while the amounts of negatively charged defect types hardly experience any increment. Only for  $s = -2\pi$  we see an increase past  $\epsilon_{bind}/k_B T \gtrsim 6.5$ . This type of charge is compatible by any vertex whether or not they exhibit any  $n$ -fold rotational symmetry. This can be realized by adding twice as much subunits around the vertex before closure. The results hint that rapid “off-target” assembly induced by large edge binding is reflected on an overabundance of topological defects. The steric interactions due to excluders introduce an additional bias for the selection of positive defects.

In Fig. 9D we show the dependence of mean graph distance to the boundary,  $\langle d_B \rangle$ , with respect to the binding

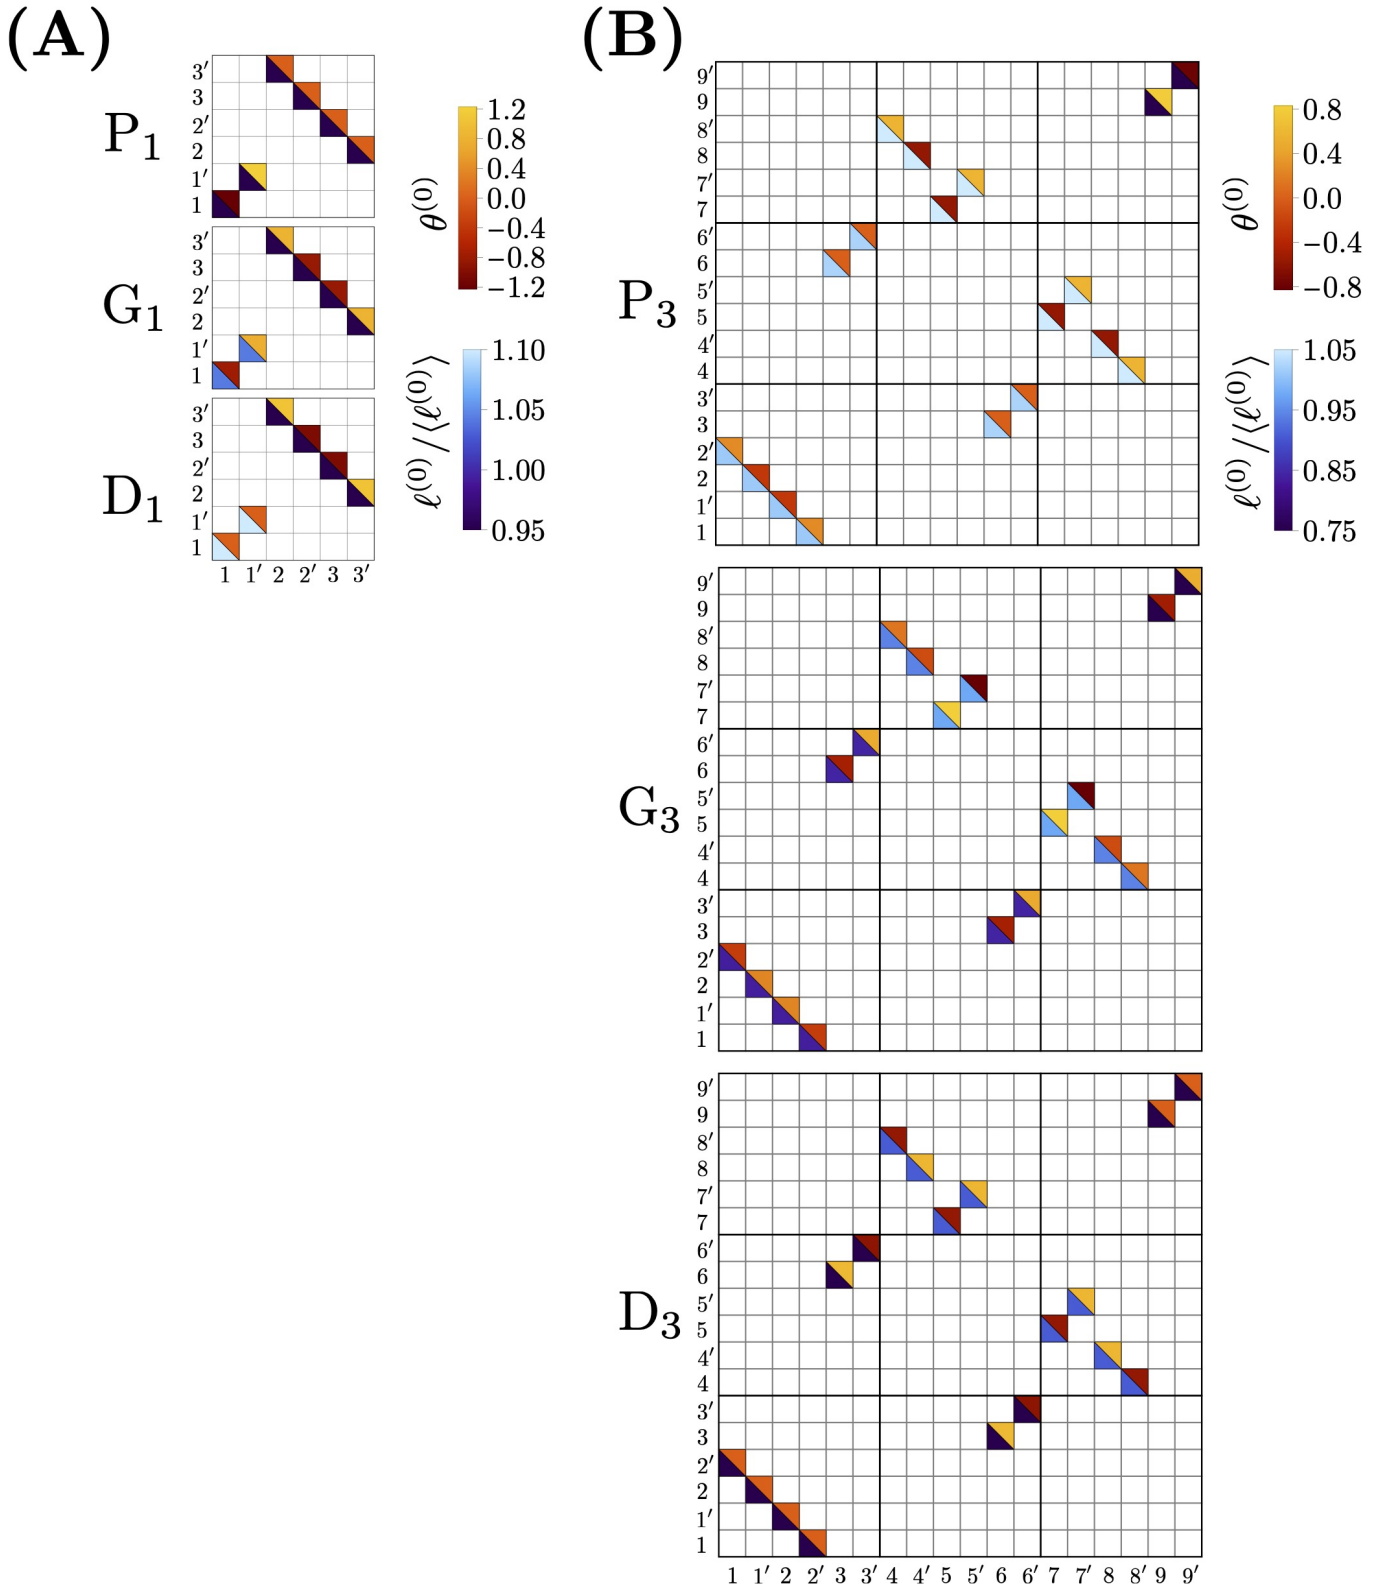

FIG. 3: (A-B) Interaction matrix for  $T=1$  and  $T=3$  structures respectively. Each colored block represents a valid edge-pairing in which The lower (upper) half color of each colored-block in the matrix represents the target length (dihedral angle) of a valid edge-pairing. Notice that the matrix “topologies” for a given triangulation number  $T$  are the same and we only need to specify the geometric data of each structure.

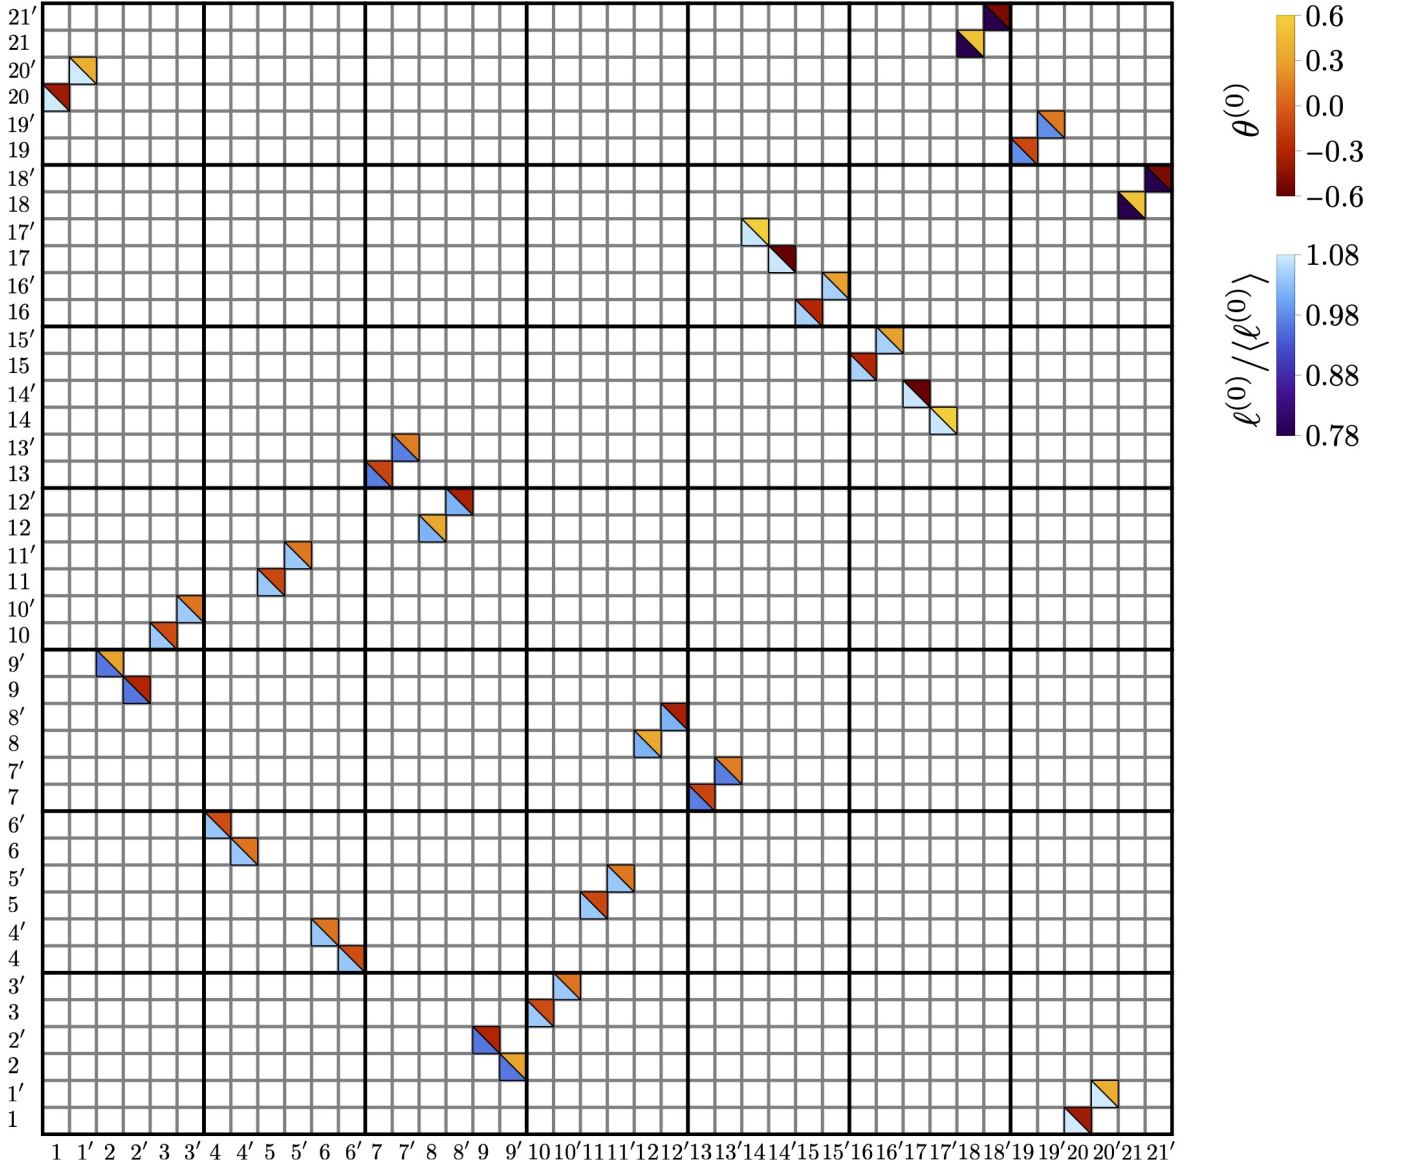

FIG. 4: Interaction matrix for  $P_7$ . Each colored block represents a valid edge-pairing in which The lower (upper) half color of each colored-block in the matrix represents the target length (dihedral angle) of a valid edge-pairing.

affinity. We perform this calculation by measuring the graph geodesic of all the vertices composing a structure to the nearest vertex located at the boundary of the structure. In order to avoid any bias coming from the starting seed, we do not include the graph distance of vertices belonging to the seed. We additionally considered the zero,  $d_B = 0$ , distance contributions of all the vertices located at the boundary of the structure. As the binding affinity increases we observe that  $\langle d_B \rangle$  increases with  $\epsilon_{\text{bind}}$ . In general, we observe that in order to accommodate the increasing number of defects, the structures adopt “stringy” morphologies like in Fig. 5C in which defects are located near the boundaries of the structure. We noticed that  $d_B \lesssim 1$  for small  $\epsilon_{\text{bind}}$  while  $d_B \lesssim 3$  for larger values of  $\epsilon_{\text{bind}}$ . Even for large  $\epsilon_{\text{bind}}$ , however, we observe that  $\langle d_B \rangle \lesssim 1$  which suggests, at least for the binding affinity range we considered, that vertices located at the boundary of the structure tend to skew  $\langle d_B \rangle$  towards smaller values regardless of the strength of the binding affinity.

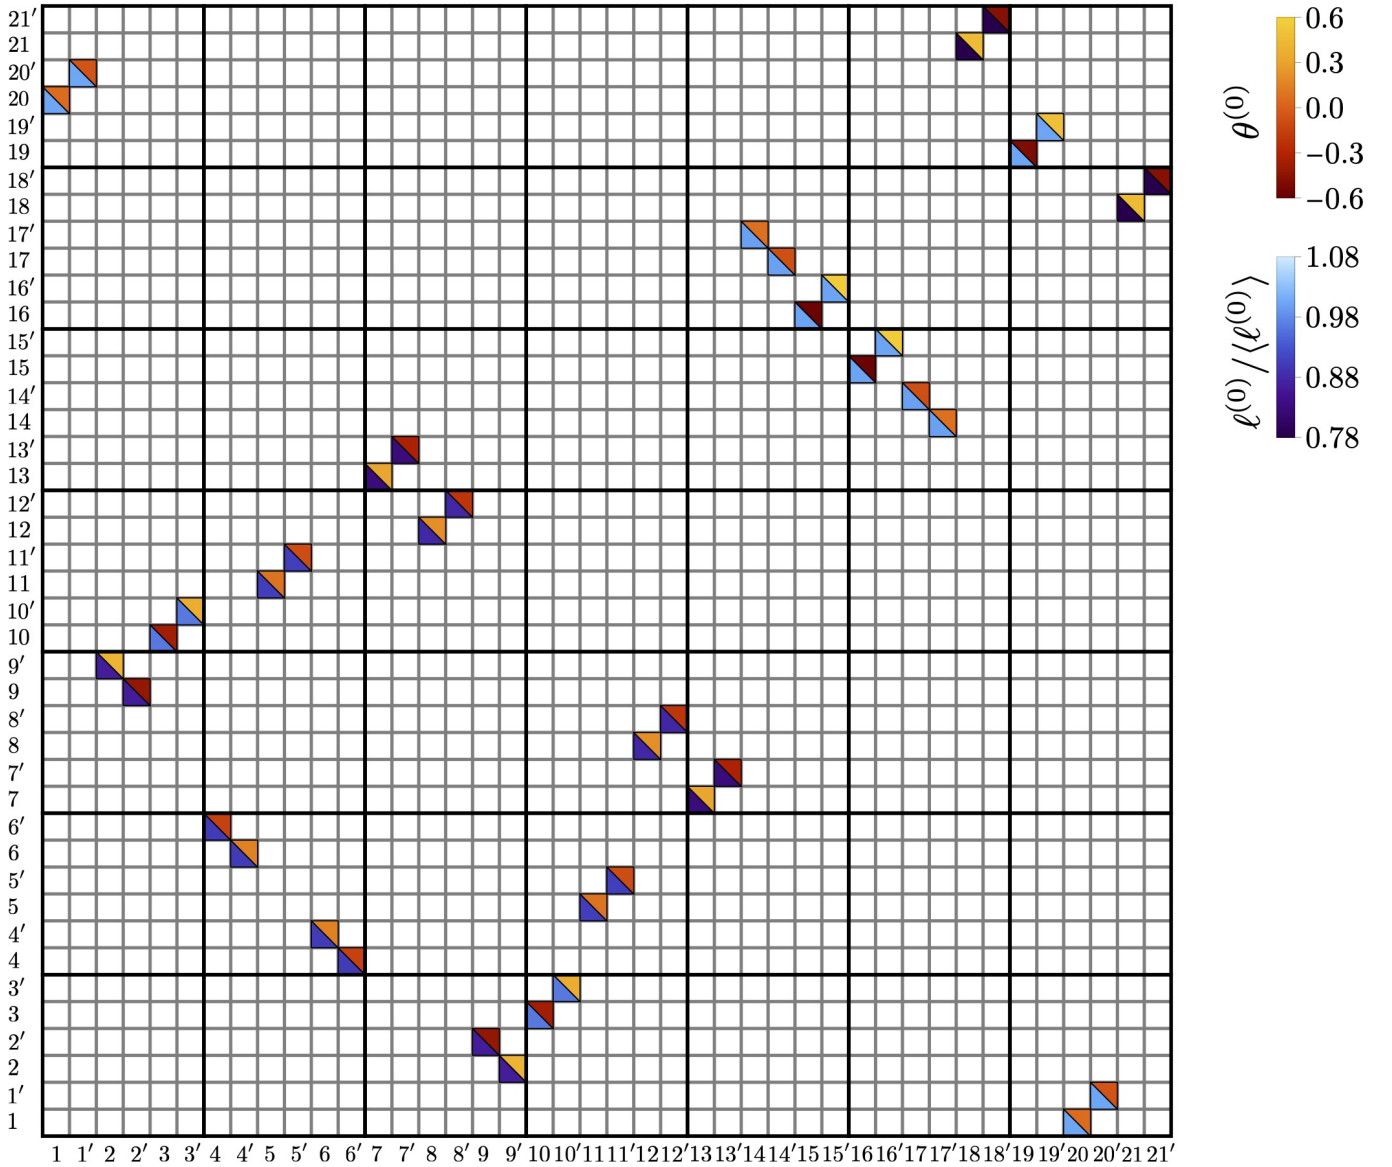

FIG. 5: Interaction matrix for G7. Each colored block represents a valid edge-pairing in which The lower (upper) half color of each colored-block in the matrix represents the target length (dihedral angle) of a valid edge-pairing.

## V. THE MODEL

In this section we provide additional details about the model and Monte Carlo simulation that we used to generate the results in the main text. The model and algorithm have been presented in ref. [3–5]. In particular, we consider flexible triangular subunits which can bind to each other along edges with a set of preferred dihedral angles that set the preferred curvatures of the assembling sheet. Monte Carlo simulations are performed in the grand canonical ensemble at fixed  $\mu VT$ , with  $\mu$  the chemical potential of subunits in the bath. Each Monte Carlo simulation involves a single cluster undergoing assembly and disassembly, with subunits taken from or returned to the bath respectively, as well as structural relaxation moves. We describe specific differences with respect to the RG model below.

### A. Energies

Each three edges of the triangular subunits may be of different types,  $t(p) = 1, 2, 3$ , for edge index  $p$  and whether a given type can bind to another type is given by the matching rules.

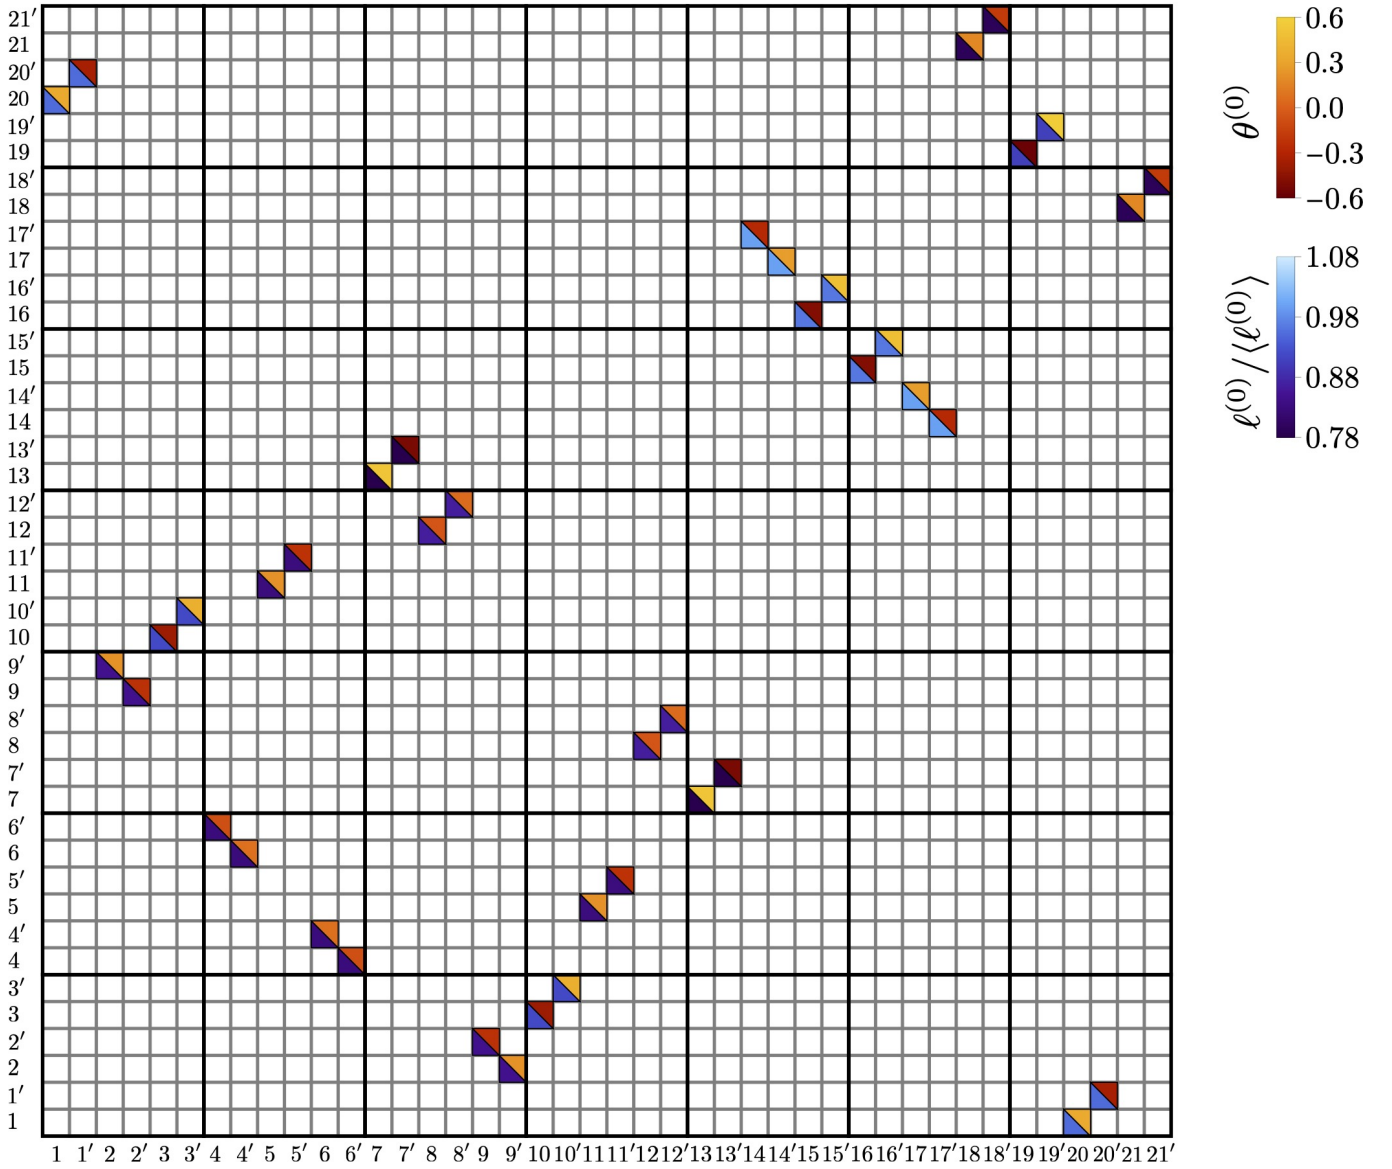

FIG. 6: Interaction matrix for D<sub>7</sub>. Each colored block represents a valid edge-pairing in which The lower (upper) half color of each colored-block in the matrix represents the target length (dihedral angle) of a valid edge-pairing.

The total energy of the system is given by

$$E = \sum_p^{3n_s} E_{\text{stretch}}^p + \frac{1}{2} \sum_{\langle pq \rangle} (E_{\text{bend}}^{pq} + E_{\text{bind}}^{pq}) \quad (1)$$

where the first sum goes over all edges, with  $n_s$  the number of subunits in the cluster. The second sum only goes over bound edges (i.e. non-boundary, adjacent edges, so there are  $2n_b$  terms in the sum, with  $n_b$  as the number of bonds). The 1/2 factor corrects for double counting.

The stretching energy is defined as:

$$E_{\text{stretch}}^p = \epsilon_s \frac{(l^p - l_0)^2}{2} \quad (2)$$

where  $\epsilon_s$  is the stretching modulus,  $l^p$  is the instantaneous length, and  $l_0$  is the stress-free (rest) length of an edge. For the tubule model we set the stretching modulus and rest length equal for all edges.

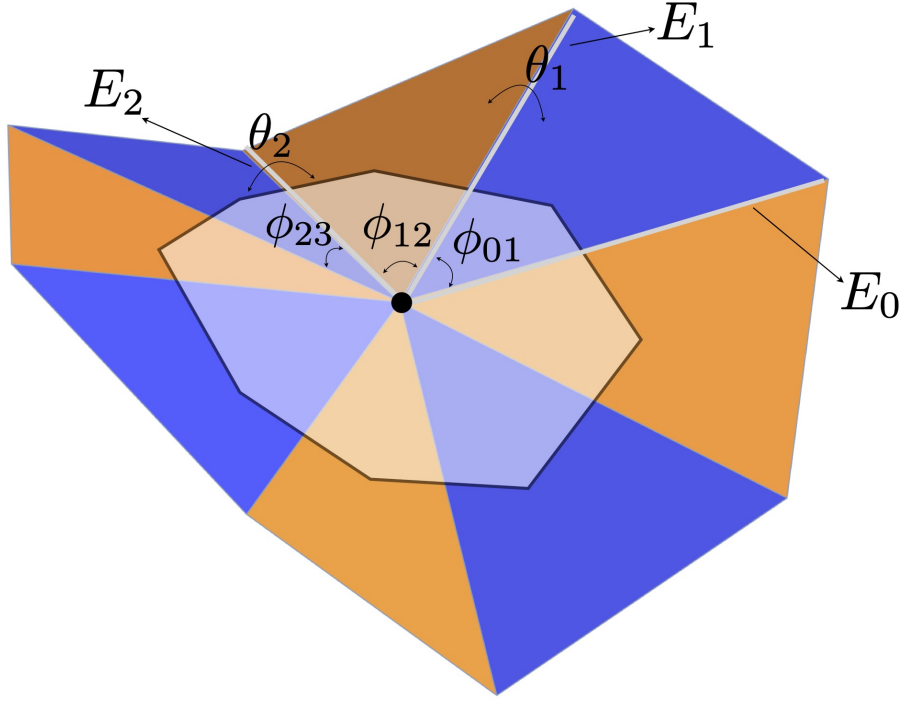

FIG. 7: Illustration of the topological charge calculation procedure: given a closed path of subunits around a vertex we can move across the anticlockwise-ordered edges,  $E_i$ , meeting at the vertex in order to determine the charge. Moving between two edges  $E_1$  and  $E_2$  an angular contribution  $\phi_{01}$  is picked up. As we move to the neighboring subunit and angle contribution corresponding to the dihedral angle is picked up as well. The process is continued until we are back at the starting subunit. Using the collection of ordered angles  $\phi_{01}, \theta_1, \phi_{12}, \theta_2, \dots$  allows us to build the rotation composition of Eq. 2. Notice that in order to find the “true” effective rotational angle  $\Phi$  we need to use the  $\phi$  and  $\theta$  angles of the “target” geometry instead of the “current” geometry.

The bending energy is quadratic in deviations from the preferred dihedral angle:

$$E_{\text{bend}}^{pq} = \kappa_b \frac{(\theta^{pq} - \theta_0^{t(p)t(q)})^2}{2} \quad (3)$$

with  $p$  and  $q$  adjacent edges and  $t(p), t(q)$  the edge types.  $\kappa_b$  is the bending modulus and is set equal for all edge types.  $\theta_0^{t(p)t(q)}$  is the preferred dihedral angle between edges with types  $t(p)$  and  $t(q)$ .

Binding energies corresponding to all matching edge pairs are set equal, to  $E_{\text{bind}}^{pq} \equiv \epsilon_b$ .

In addition to the above terms, each subunit has at its center of mass a spherical excluder of radius  $0.2l_0$  to prevent subunit overlaps. Finally, to prevent extreme distortions of subunits, maximum edge length fluctuations are limited to  $l_0/2 < l < 3l_0/2$ .

## B. Coarse-graining

Our model is motivated by the triangular DNA origami subunits developed in Sigl et al.[6], in which subunits bind through lock-and-key ‘patches’ along subunit edges in which attractive interactions are generated through blunt-end stacking of unsatisfied nucleotides. Therefore, in our model we define attractive bonds along subunit edges (rather than at vertices as in the RG model). In particular, attractive bonds occur at each shared pair of subunit edges with the same type. Because the interactions in the experimental system are driven by nucleotide stacking, they are extremely short-ranged in comparison to the subunit size (the subunit edge lengths are approximately 60 nm). Therefore, in our simulations we avoid resolving the short length scale fluctuations in separation distance between bound edges and their associated vertices by coarse-graining as follows.

A microstate  $i$  is defined as the position of all the  $3n_s$  vertices of  $n_s$  subunits:  $i \rightarrow (\vec{x}_1, \vec{x}_2, \dots, \vec{x}_{3n_s})$  The grand

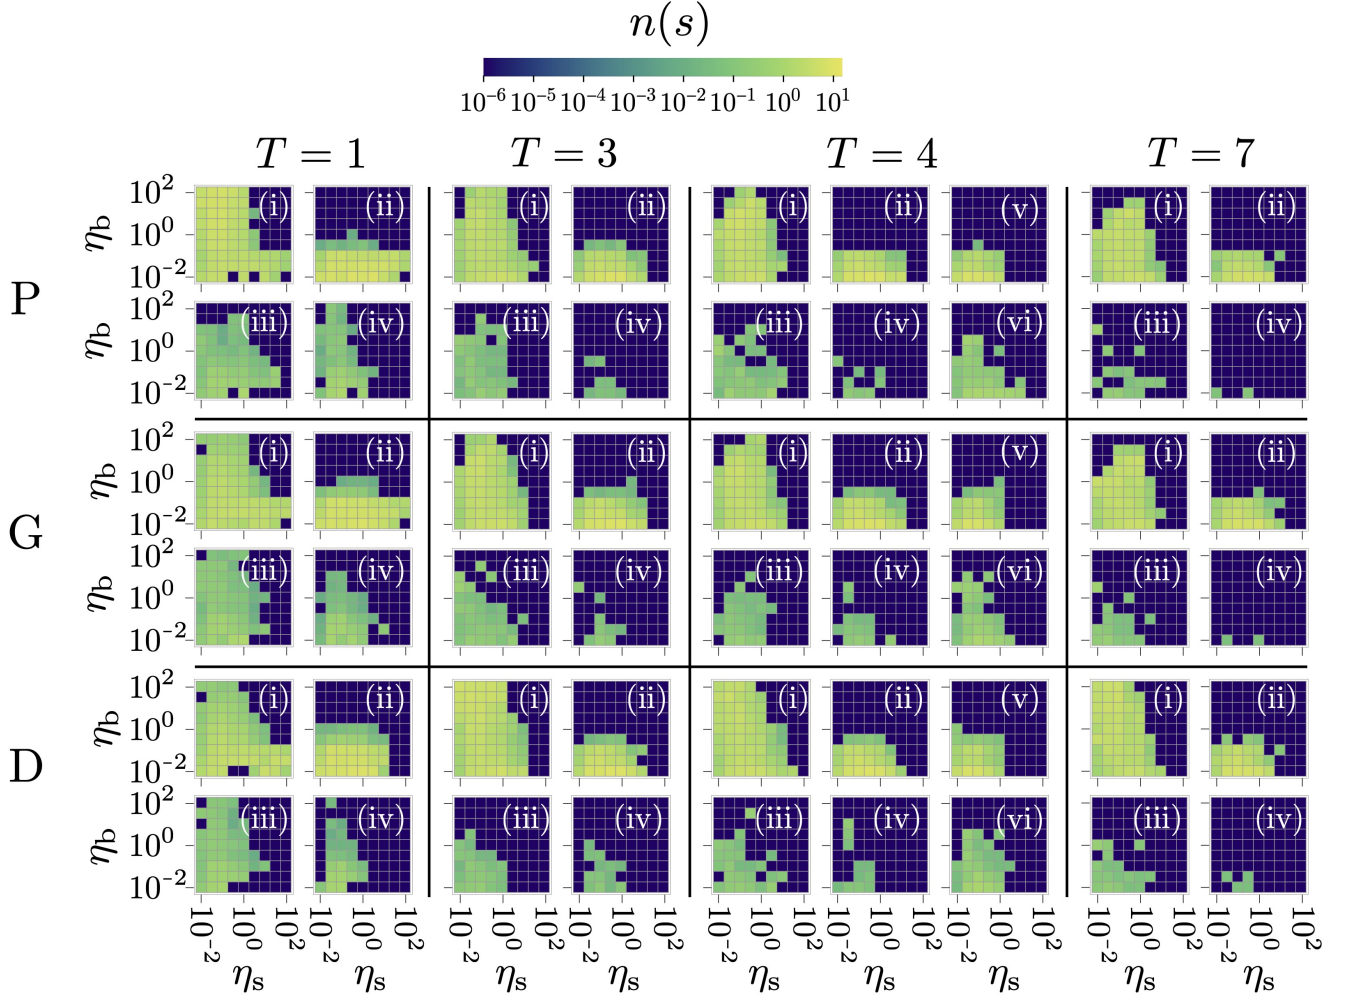

FIG. 8: Defect population per unit cell,  $n(s)$ , as a function of dimensionless ratios  $\eta_s$  and  $\eta_b$  for each of the defect types. Panels (i) to (vi) respectively correspond to charges  $+2\pi/3$ ,  $+\pi$ ,  $-2\pi/3$ ,  $-\pi$ ,  $+\pi'$ , and  $-\pi'$ .

canonical probability *density* of finding the system around state  $i$  is

$$f(i) = \frac{P(\vec{x}_1, \vec{x}_1 + d\vec{x}_1; \dots; \vec{x}_{n_s}, \vec{x}_{n_s} + d\vec{x}_{n_s})}{d\vec{x}_1 d\vec{x}_2 \dots d\vec{x}_{3n_s}} = \frac{1}{Z_\Omega} \frac{e^{\beta n_s \mu}}{\lambda^{9n_s}} e^{-\beta E_i} \quad (4)$$

where  $\mu$  is the chemical potential and  $\lambda^3$  is the standard state volume. This probability density has the dimensions of  $1/\text{volume}^{3n_s}$  corresponding to all the  $3n_s$  vertices of the subunits. Due to bonds, however, some pairs of vertices are confined within a *binding volume*  $v_a$ . We consider a square-well potential so that the binding energy is constant within this volume. Analogous to Ref. [7], we can then coarse-grain to avoid resolving intra-bond fluctuations. We assume that fluctuations of bound edges are sufficiently small that each pair of vertices at either end of a bound edge pair are constrained within a *binding volume*  $v_a$ . Note that we constrain vertices rather than edges so that the coarse-grained microstate can be represented in terms of positions of vertices rather than edges, which is easier to implement computationally. In the coarse-grained system, a coarse microstate is specified by the coordinates corresponding to the independent vertex degrees of freedom (with 1 degree of freedom for each bound vertex group and unbound vertex):  $\Gamma \rightarrow (\vec{x}_1, \vec{x}_2, \dots, \vec{x}_{n_v})$ , where  $n_v$  is the number of independent bound vertex groups and free vertices. The probability of such a coarse-grained state is given by the net weight of all the corresponding fine-grained microstates:

$$\rho(\Gamma) = \int_{\{v_a\}} f(i) d^{n_{vB}} \vec{x} \quad (5)$$

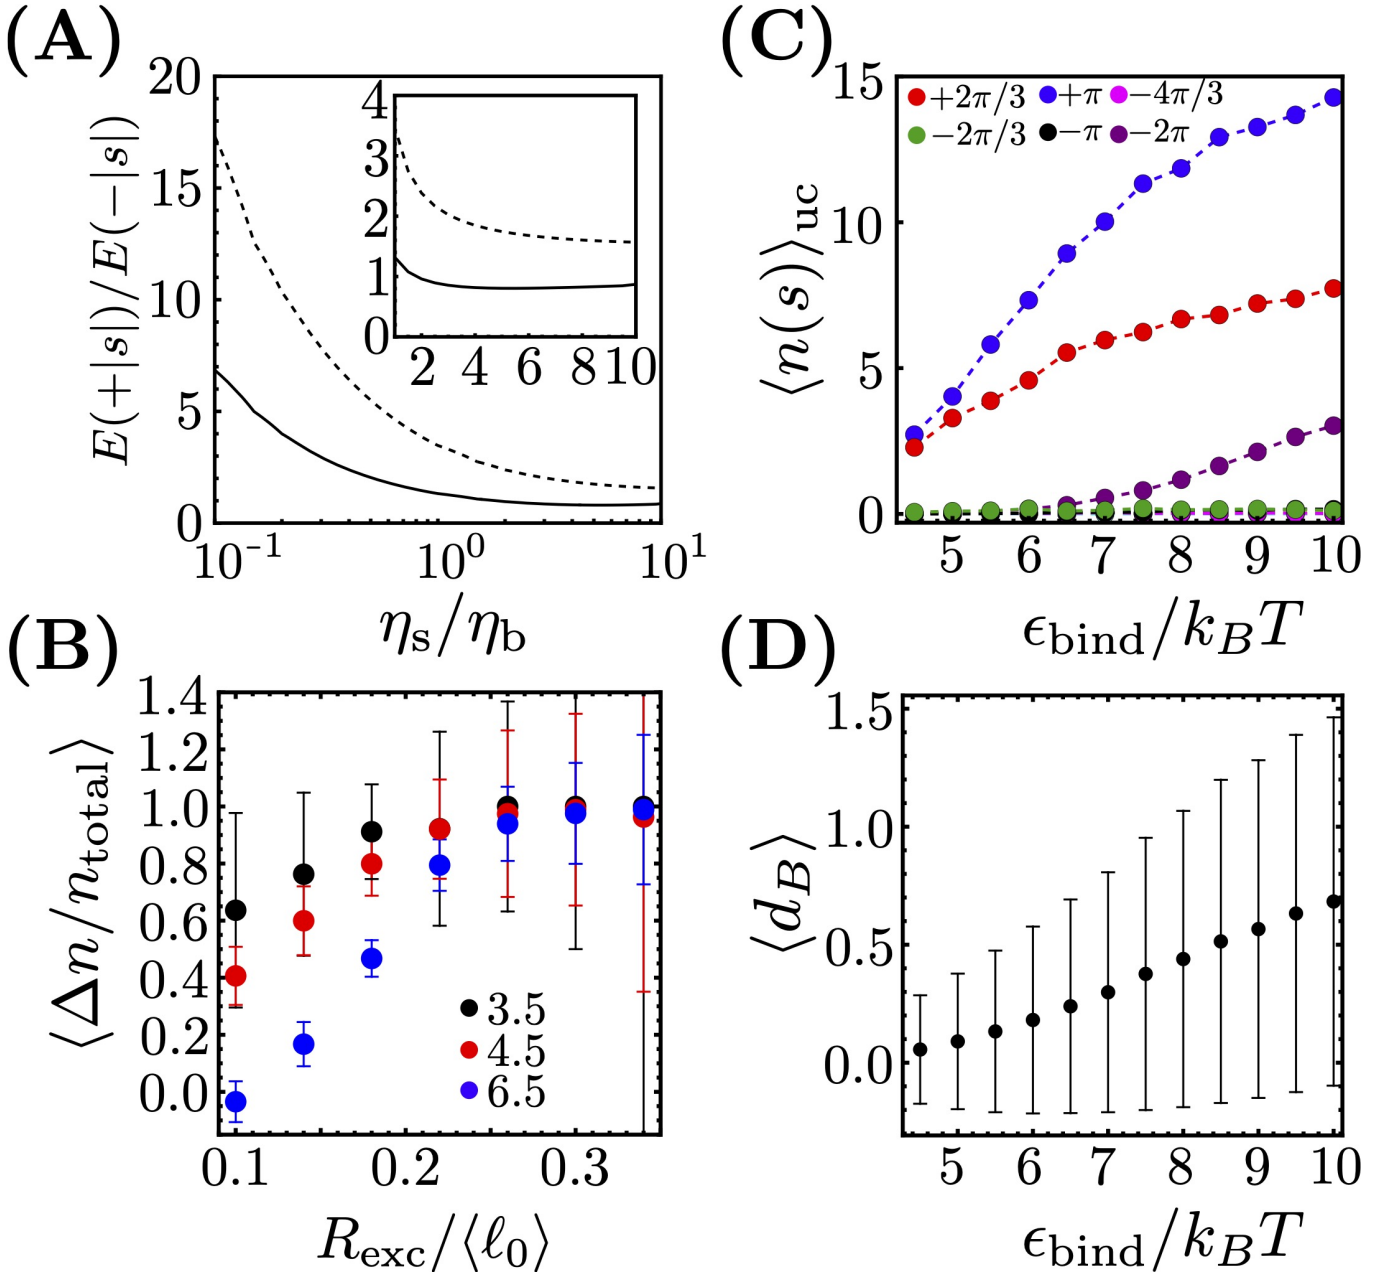

FIG. 9: **(A)** Elastic energy ratio  $E(+|s|)/E(-|s|)$  for  $|s| = 2\pi/3$  (solid line) and  $|s| = \pi$  (dashed line) as a function of  $\eta_s/\eta_b$ . **(B)** Mean relative counts difference between positive and negative charges,  $\langle \Delta n/n_{\text{total}} \rangle$ , for increasing excluder radius size. The black, red, and blue points correspond to fixed binding affinity values  $\epsilon_{\text{bind}} = 3.5, 4.5$ , and  $6.5$  respectively. **(C)** Mean defect type population per unit cell,  $\langle n(s) \rangle_{\text{uc}}$ , for a  $G_7$  structure for increasing binding affinity,  $\epsilon_{\text{bind}}$ . The elastic moduli are fixed for all points and calculated using  $\eta_s = 1$  and  $\eta_s = 0.01$  with a reference value  $\epsilon_{\text{bind}} = 6.5k_B T$ . The chemical potential,  $\mu = -4.5k_B T$ , is also fixed for all points. Each point is computed as the mean of 50 independent realizations. **(D)** Mean graph distance,  $\langle d_B \rangle$ , for increasing binding affinity and same simulations parameters of **(C)**.

where  $n_{\text{VB}}$  is the number of vertex-bonds and is given by  $n_{\text{VB}} = 3n_s - n_v$ . For simplicity, we take the limit in which  $\sqrt[3]{v_a}$  is small in comparison to the length scale over which the elastic energy varies, so that the energy is constant within the bound volume  $v_a$ . Then  $f(i)$  is a constant, and the probability density is given by

$$\rho(\Gamma) = \frac{1}{Z_\Omega} v_a^{n_{\text{VB}}} \frac{e^{\beta n_s \mu}}{\lambda^{9n_s}} e^{-\beta E_\Gamma} \quad (6)$$

where  $E_\Gamma$  is the total energy of state  $\Gamma$  (including stretching, bending and binding energies). The coarse graining

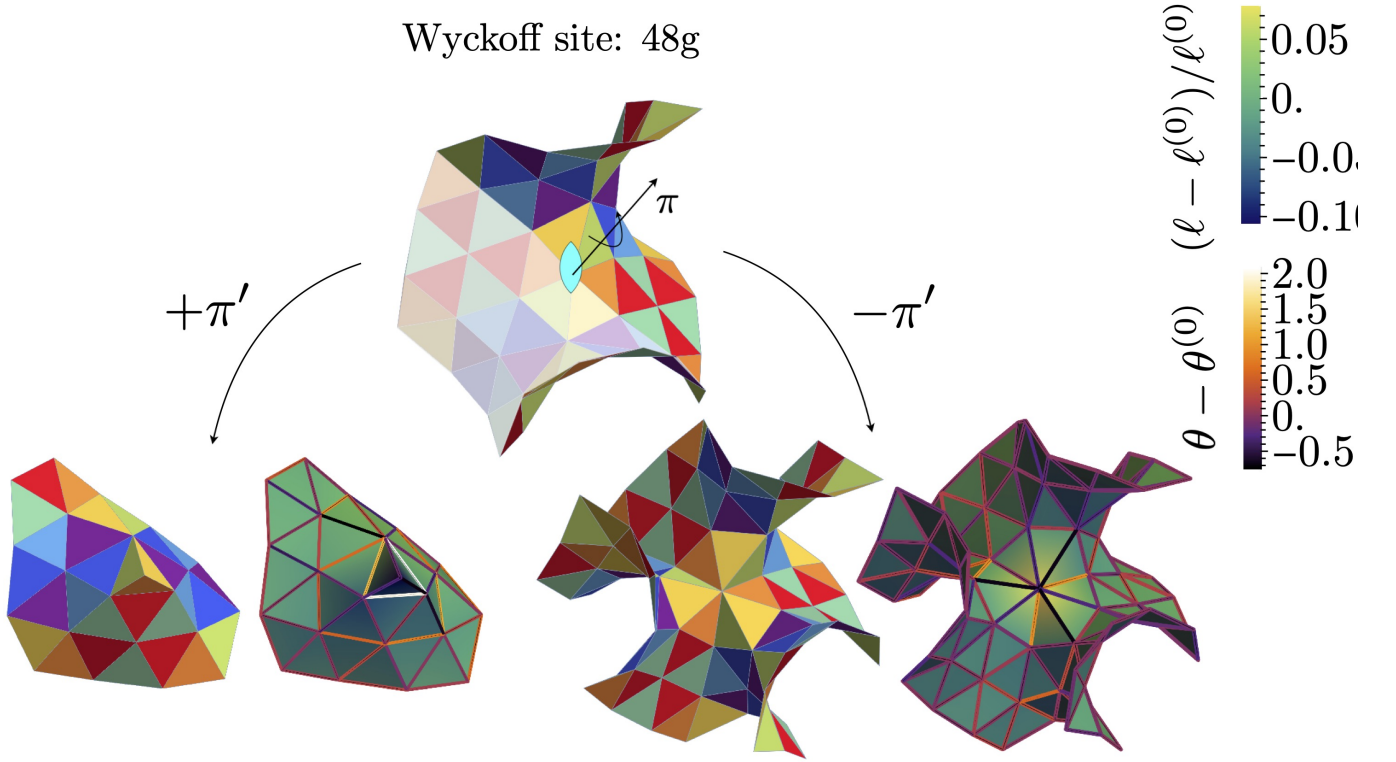

FIG. 10: For a subset of  $T$  values additional Wyckoff sites with a 2-fold symmetry can be found. The triangulation on top shows a defectless patch exhibiting a Wyckoff site 48g present in  $G_4$  structures. Defects of charge  $s = \pm\pi$  are generated through a Volterra construction on the defectless patch. The charges are primed to distinguish them from the defects obtained through the Wyckoff sites 24d. Each defective patch is colored with respect to the unique triangle ID label as shown on the left patches as well as their length strain (faces) and angle strain (edges) as shown on the right patches.

process is illustrated in Fig. 12.

### C. Implementation and data structure

The simulation is implemented on top of the OpenMesh library [8]. Subunits are implemented as triangular mesh elements. OpenMesh uses the halfedge data structure which is suitable to implement triangles with directed normals (Fig 13). The directed halfedges allow for a clockwise iteration through the boundary of a triangle, which makes the two faces of the triangles distinguishable. Only halfedges with opposite orientations can bind together, making it impossible to form a Mobius strip, for example. The data structure and the resulting iterators in OpenMesh allow for an easy and efficient iteration over the neighborhood of mesh elements (vertices, edges and faces). The implementation of mesh element rearrangements is less straightforward, but we implemented it via the insertion and removal of virtual triangles. In addition, OpenMesh allows for the storage of various properties on mesh elements, allowing storage of edge types and face types stored on the elements. To improve readability in the upcoming sections, we will not represent halfedges separately.

## VI. THE MONTE CARLO MOVES

In this section we detail the Monte Carlo moves of the simulation. Our algorithm has 11 moves: vertex displacement, simple subunit insertion/deletion, wedge insertion/deletion, wedge fusion/fission, crack fusion/fission, and edge fusion/fission.

*Detailed balance.* For the transition between state  $\Gamma$  and  $\Gamma'$  detailed balance corresponds to [7, 9]:

$$P(\Gamma) \times \alpha(\Gamma \rightarrow \Gamma') \times p_{\text{acc}}(\Gamma \rightarrow \Gamma') = P(\Gamma') \times \alpha(\Gamma' \rightarrow \Gamma) \times p_{\text{acc}}(\Gamma' \rightarrow \Gamma) \quad (7)$$

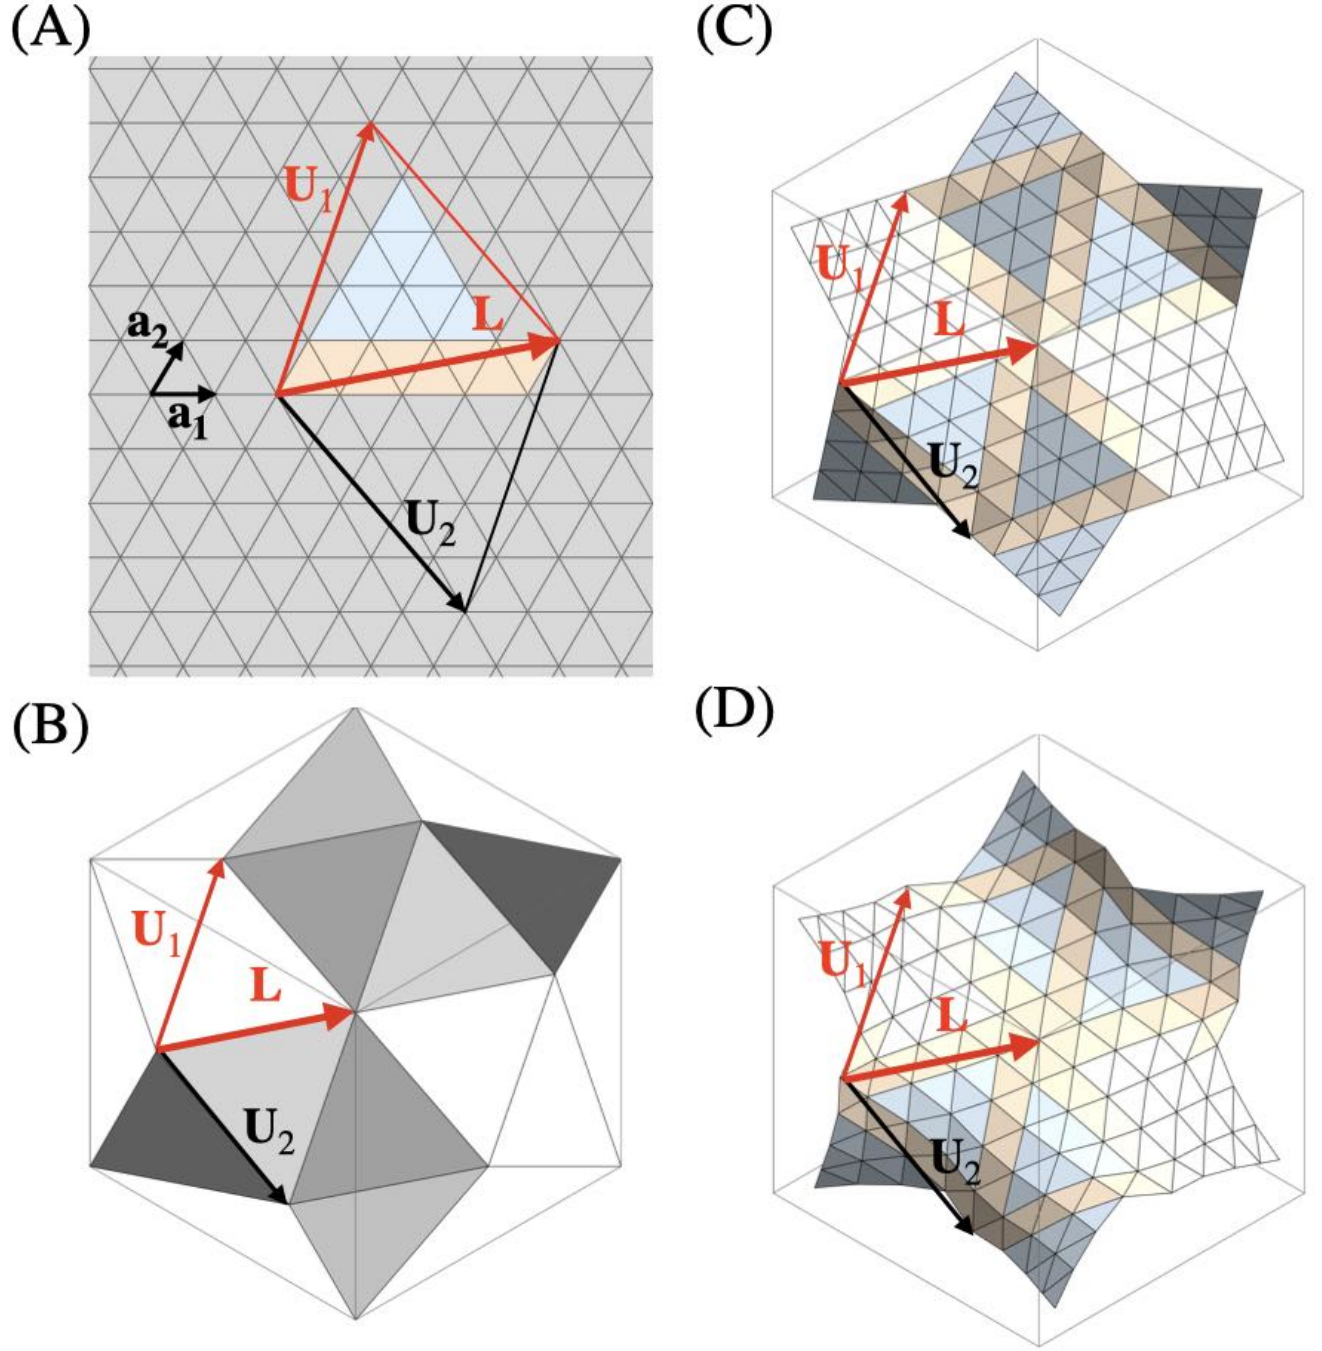

FIG. 11: Construction of triangulation for given  $T$  from  $T = 1$  triangulation. (A) A planar construction defines the vectors  $\mathbf{L}$ ,  $\mathbf{U}_1$ ,  $\mathbf{U}_2$  in terms of the triangular lattice vectors  $\mathbf{a}_1$ ,  $\mathbf{a}_2$ . The lattice triangles contained in the larger triangle with edges  $\mathbf{L}$ ,  $\mathbf{U}_1$  (blue) will be mapped to each face and the lattice triangles that contain the line segment  $\mathbf{L}$  (orange) will be mapped to each edge of the base ( $T = 1$ ) triangulation. Here, the construction is illustrated for  $(h, k) = (4, 1)$ . (B) The base triangulation is a set of triangles so that each triangle has three neighbors and a consistent orientation can be assigned to the triangulation. Here, the unit cell of the  $T = 1$  triangulation associated with the gyroid surface is shown, deriving from the surface's asymmetric units. (C) The triangles of the planar construction are mapped to the base triangulation by identifying each edge with the triangulation vector  $\mathbf{L}$  and associated neighboring edges  $\mathbf{U}_1$ ,  $\mathbf{U}_2$ . (D) Finally, the vertices are translated closer to the surface while maintaining the targeted symmetries of the structures.

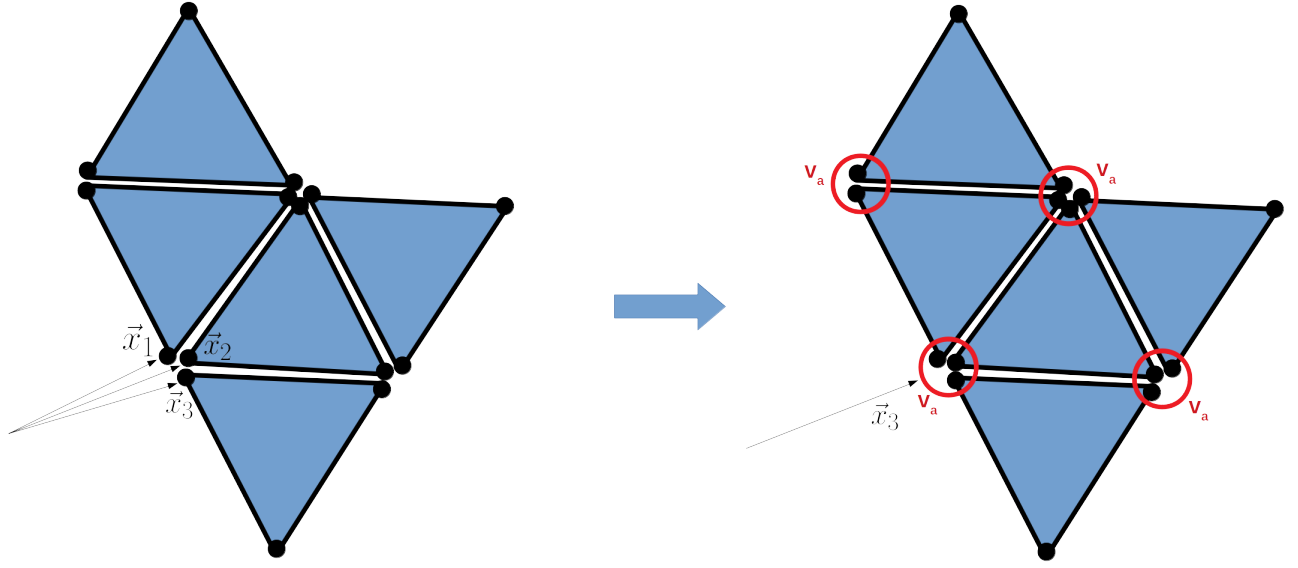

FIG. 12: Coarse-graining of an example cluster configuration. In this configuration, the number of subunits is  $n_s = 5$ , the number of initial (before coarse-graining) vertices is  $3n_s = 15$ , and the number of vertices after coarse-graining is  $n_v = 7$ . The red circles indicate bound vertex groups, and the number of vertex degrees of freedom that have been eliminated by coarse-graining in this configuration is  $n_{VB} = 1 + 3 + 2 + 2 = 8 = 3n_s - n_v$ . Motivated by DNA origami subunits in Sigl et al. [6], the attractive interactions (i.e. ‘bonds’) in this model occur along edge-pairs of the same type shared by two subunits. In this configuration there are  $n_b = 4$  bonds.

where  $\alpha(\Gamma \rightarrow \Gamma')$  is the probability of generating a  $\Gamma \rightarrow \Gamma'$  move attempt (trial),  $p_{\text{acc}}(\Gamma \rightarrow \Gamma')$  is the probability of accepting the move, and  $P(\Gamma) = \rho(\Gamma) d^{n_v(\Gamma)} \vec{x}$  is the equilibrium probability of finding a system in a voxel of volume  $d^{n_v(\Gamma)} \vec{x}$ .

Next, we use Eq. (7) to define the acceptance criteria for each MC move. The acceptance criteria are derived in detail for the wedge fusion/fission move; the steps to follow are the same for all other moves.

### A. Vertex displacement

In this move, a vertex is randomly selected, a random uniform displacement is drawn, and the vertex is displaced to its new position according to:

$$x \rightarrow x + \mathcal{U}(-d_{\text{max}}, d_{\text{max}}) \quad (8)$$

$$y \rightarrow y + \mathcal{U}(-d_{\text{max}}, d_{\text{max}}) \quad (9)$$

$$z \rightarrow z + \mathcal{U}(-d_{\text{max}}, d_{\text{max}}) \quad (10)$$

with  $d_{\text{max}}$  the maximum displacement. The move is accepted with a probability  $p_{\text{acc}} = \exp(-\Delta E/k_B T)$  where  $\Delta E$  is the (bending plus stretching) energy change due to the displacement. The parameter  $d_{\text{max}}$  can be adjusted during a burn-in period to optimize convergence to equilibrium. Generally optimal values are on the order of the typical length scale of thermal fluctuations dictated by the elastic energy, leading to acceptance probabilities on the order of 50%. In our simulations typical values are between  $d_{\text{max}} = [0.01l_0, 0.1l_0]$ . The vertex displacement move is illustrated in Fig 14: the number of subunits  $n_s$ , number of vertices  $n_v$ , number of vertex bonds  $n_{VB}$  and number of bonds  $n_b$  remains unchanged during this move.

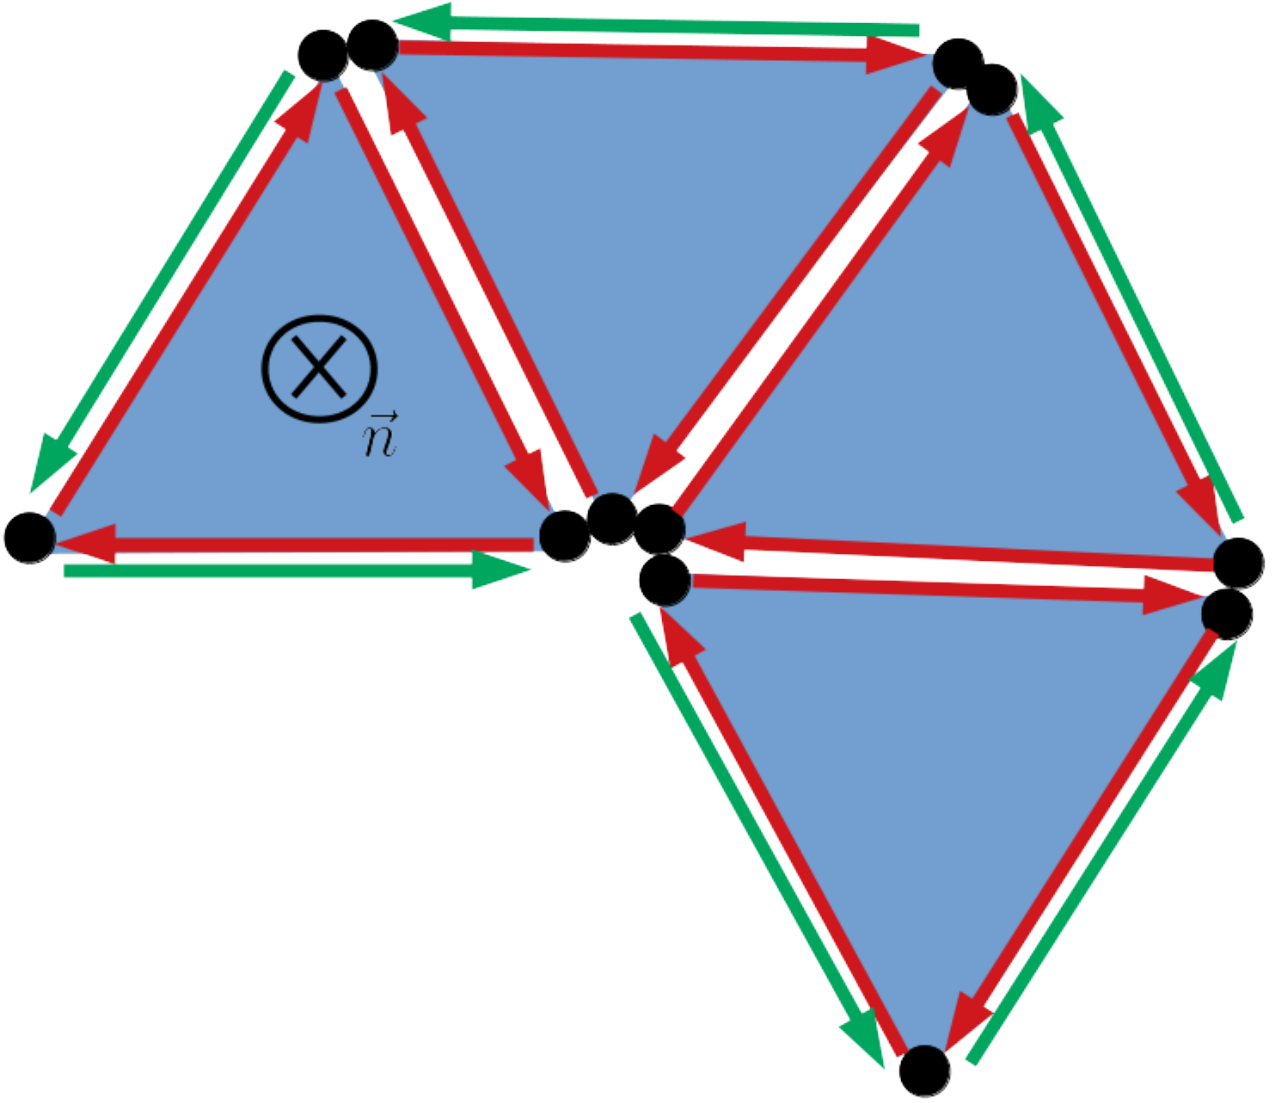

FIG. 13: The halfedge data structure used by OpenMesh. Each edge is represented by two directed edges. Boundary edges are no exception and thus are represented by a non-boundary halfedge and a boundary halfedge (in green). This latter is irrelevant for our model. Directed edges allow for the unambiguous definition of face normals, for efficient iterations of the element's neighborhood as well as boundary iterations.

## B. Simple insertion / removal

### 1. Simple insertion

In this move, an edge is randomly selected from the set of all boundary edges, where a new subunit will be attached. The number of such boundary edges is  $n_e$ . Subunits can be inserted in  $n_r$  different rotations, where  $n_r$  is the number of distinct rotational states for a subunit which has one edge aligned with the edge of a neighboring subunit. For our triangular subunits with three distinct edge types,  $n_r = 3$ . In our algorithm, during insertion of a subunit its rotational state is chosen randomly from the set of three possibilities. If the aligned edge is not complementary to the type of the boundary edge, then the move is rejected. In this work, the two edges must be of the same type to be complementary.

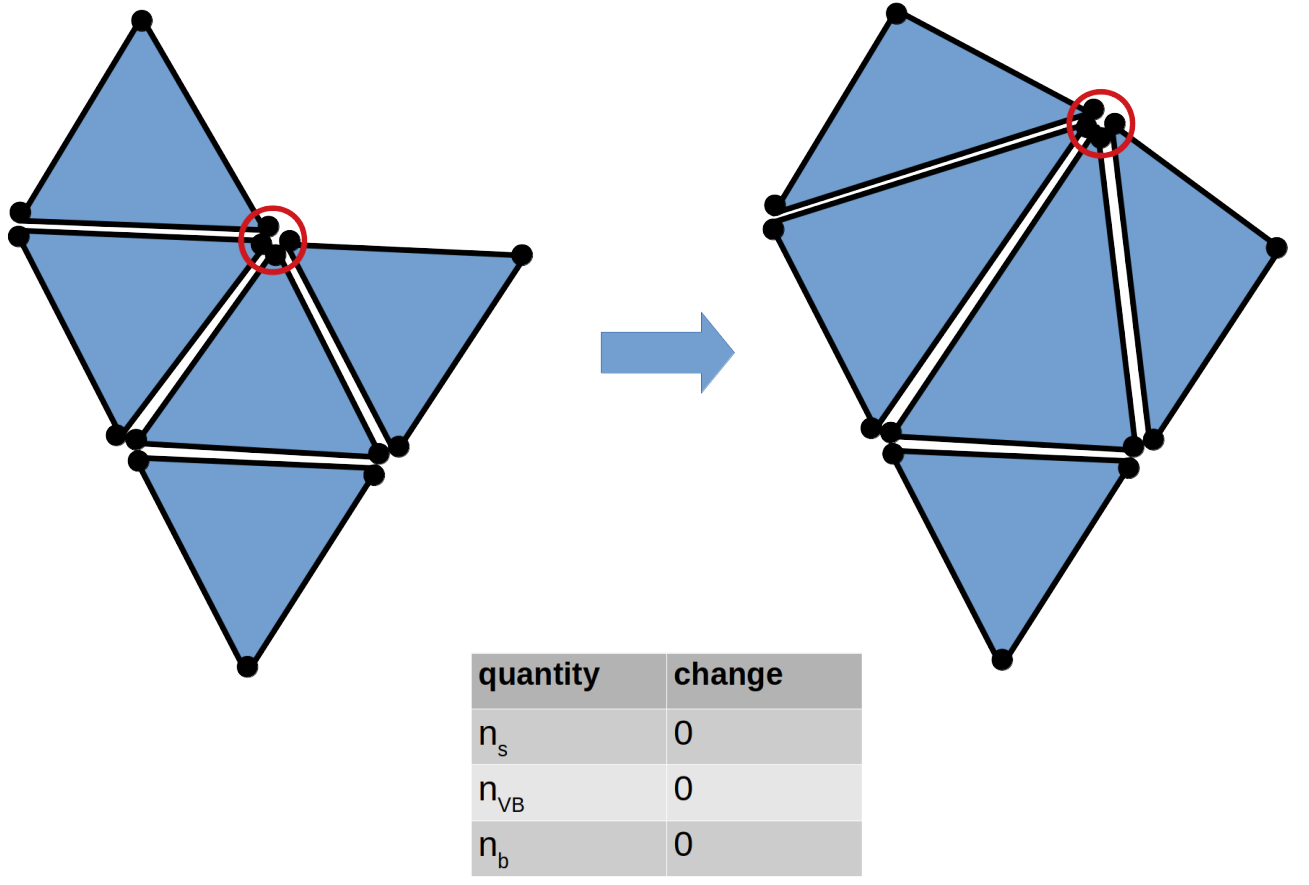

FIG. 14: Vertex move. A vertex is randomly displaced and the move is accepted according to the usual Metropolis probability.

The positions of two of the new subunit's vertices (those at either end of the edge being bound) are set equal to the positions of the corresponding vertices of the boundary edge to which it is binding. The third vertex position is randomly chosen from within a volume  $v_{\text{add}}$  centered at the equilibrium position of the new vertex.

Thus, the attempt probability for a simple insertion is given by:

$$\alpha(i \rightarrow j) = n_e k_i \tau n_r \times \frac{1}{n_e n_r (v_{\text{add}}/d\vec{x})}. \quad (11)$$

Then, applying Eq. (7) and the attempt probability for the reverse move (simple deletion, presented next, Eq. (13)), the acceptance probabilities for a simple insertion is

$$p_{\text{acc}}(i \rightarrow j) = \min \left[ 1, \frac{v_a^2 v_{\text{add}}}{\lambda^9} \exp[-(\Delta E_{i \rightarrow j} - \mu)/k_B T] \right]. \quad (12)$$

$\Delta E_{i \rightarrow j}$  is the energy change due to the move and includes the stretching energy of the newly inserted subunit, its bending energy along the shared edge, and the binding energy due to the creation of an extra bond. During this move, one new (edge) bond and two new vertex bonds are created; i.e.  $n_b \rightarrow n_b + 1$  and  $n_{VB} \rightarrow n_{VB} + 2$ . Moreover, the number of vertices in the structure increases by one,  $n_v \rightarrow n_v + 1$ .

## 2. Simple removal

The reverse move to simple insertion is simple removal. Subunits that can be deleted with this move are those with two boundary edges. The number of simply removable subunits is  $n_{\text{sr}}$ . One of these is selected randomly, so the

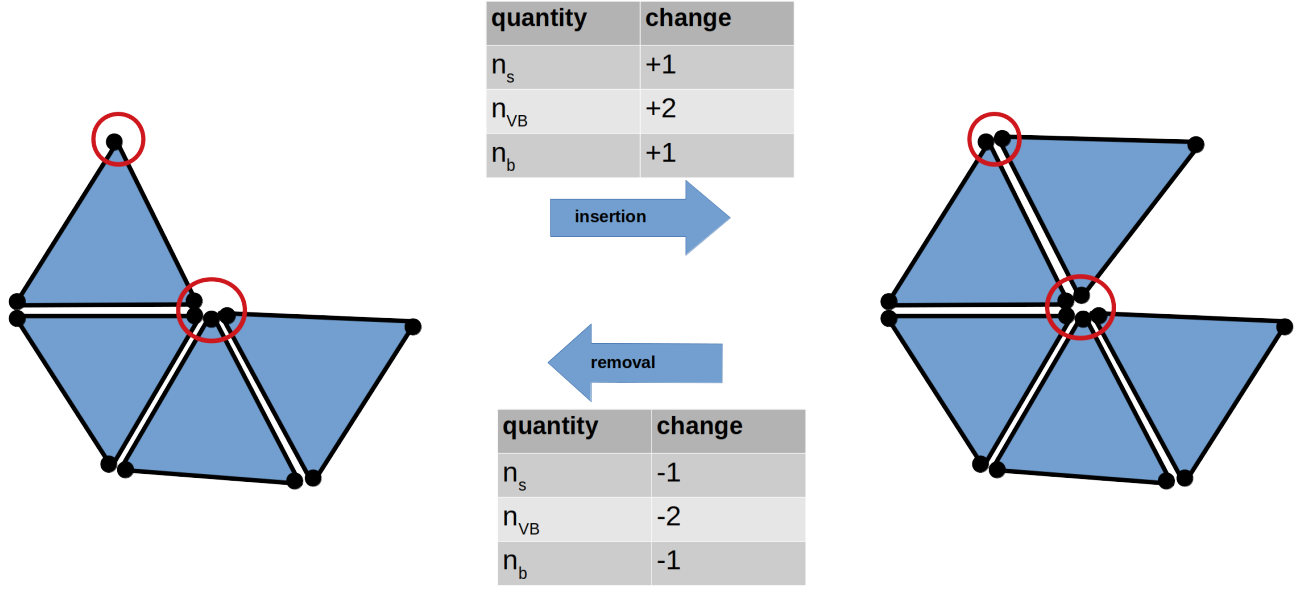

FIG. 15: Simple insertion and removal.

attempt probability is

$$\alpha(j \rightarrow i) = n_{sr} k_i \tau \times \frac{1}{n_{sr}} \quad (13)$$

and, using Eq. (7) and Eq. (11), the acceptance probability is

$$p_{acc}(j \rightarrow i) = \min \left[ 1, \frac{\lambda^9}{v_a^2 v_{add}} \exp[-(\Delta E_{j \rightarrow i} + \mu)/k_B T] \right] \quad (14)$$

During this move, the structure loses one (edge) bond and two vertex bonds;  $n_b \rightarrow n_b - 1$  and  $n_{vB} \rightarrow n_{vB} - 2$ . The number of vertices in the structure decreases by one,  $n_v \rightarrow n_v - 1$ .

If there are multiple species with chemical potentials  $\mu_k$ , detailed balance must be satisfied for each species, individually. Moreover, each species can have different insertion rates  $k_i^k$ .

To keep  $\alpha < 1$ , we ensure that the insertion rate  $k_i$  constrained by

$$n_e k_i \tau n_r < 1 \quad (15)$$

$$n_{sr} k_i \tau < 1 \quad (16)$$

In equilibrium, one can use adaptive rates, i.e. reduce  $k_i$  on the run if the above condition is not satisfied. In that case, sampling is not taken for the ensuing several time steps. Alternatively, the rates may be set to a low enough value from the beginning and only tested on the run to ensure that the  $\alpha < 1$  condition is satisfied. This latter technique is appropriate for dynamical runs as it keeps the rates constant throughout the simulation.

Moreover, we must ensure that  $v_{add}$  is large enough so that the vertex does not leave the  $v_{add}$  volume during structural relaxation moves; otherwise the insertion/deletion moves would not be reversible and the detailed balance would be violated. For a better convergence, one could choose a gaussian distribution  $\mathcal{N}(\vec{r})$  for the position of the new vertex instead of a uniform distribution  $1/v_{add}$ . In this case, this distribution has to be accounted for in the acceptance probabilities  $p_{acc}(i \rightarrow j)$  and  $p_{acc}(j \rightarrow i)$ .

### C. Wedge insertion/removal

#### 1. Wedge insertion

Wedges are positions in the structure where a triangle can be inserted via attaching to two edges (Fig. 16). In a wedge move, we pick randomly from the set of available wedge positions in the structure, and pick a random orientation for the new subunit. Denoting the number of wedge positions in a given structure as  $n_w$ , the attempt probability for a wedge move is

$$\alpha(i \rightarrow j) = n_w k_i \tau n_r \times \frac{1}{n_r n_w} \quad (17)$$

In contrast to the simple insertion move, there is no need for random vertex displacement in a wedge move because all three vertices of the new subunit are fixed by the three vertices of the wedge position. Combining Eq. (17) and the attempt probability for wedge removal (Eq. (19)), The acceptance probability for a wedge insertion is

$$p_{\text{acc}}(i \rightarrow j) = \min \left[ 1, \frac{v_a^3}{\lambda^9} \exp[-(\Delta E_{i \rightarrow j} - \mu)/k_B T] \right]. \quad (18)$$

During a wedge insertion, two edge bonds and three vertex bonds are created; i.e.,  $n_b \rightarrow n_b + 2$  and  $n_{VB} \rightarrow n_{VB} + 3$ , but the number of vertices is unchanged,  $n_v \rightarrow n_v$ .  $\Delta E_{i \rightarrow j}$  includes the binding energy of the two newly formed bonds, the two bending energies along the two newly bound edges and the stretching energy of the newly inserted subunit.

#### 2. Wedge removal

The reverse move of wedge insertion is wedge removal. In a wedge removal, we randomly choose one of the removable wedges from a given structure. With the number of removable wedges as  $n_{wr}$ , the attempt probability is

$$\alpha(j \rightarrow i) = n_{wr} k_i \tau \times \frac{1}{n_{wr}}. \quad (19)$$

Using Eq. (17), the acceptance probability for a wedge removal is then

$$p_{\text{acc}}(j \rightarrow i) = \min \left[ 1, \frac{\lambda^9}{v_a^3} \exp[-(\Delta E_{j \rightarrow i} + \mu)/k_B T] \right]. \quad (20)$$

We have the following constraints on rates  $k_i$  for wedge insertion/removal:

$$n_w k_i \tau n_r < 1 \quad (21)$$

$$n_{wr} k_i \tau < 1 \quad (22)$$

As for simple insertion and removal, in the case of multiple species, detailed balance is satisfied for each species separately for wedge insertion/removal.

### D. Wedge fusion / fission

#### 1. Wedge fusion

In this move, a *fusable wedge* is closed, without inserting a new subunit (Fig 17). That is, the two vertices on either side of the wedge opening are merged into a single vertex. Fusible wedges are vertex pairs that i) form a wedge (as in the case of wedge insertion) and ii) are within a separation distance of  $l_{\text{fuse}}$ .

Denoting the number of fusible wedge positions as  $n_w$ , in each MC step, a wedge fusion is attempted with probability  $n_w k_{wf} \tau$ , where  $k_{wf}$  is an adjustable parameter controlling the relative probability of attempting wedge fusion. Then, a wedge position is selected randomly from the set of all  $n_w$  fusible wedges. The attempt probability is thus

$$\alpha(i \rightarrow j) = n_w k_{wf} \tau \times \frac{1}{n_w}. \quad (23)$$

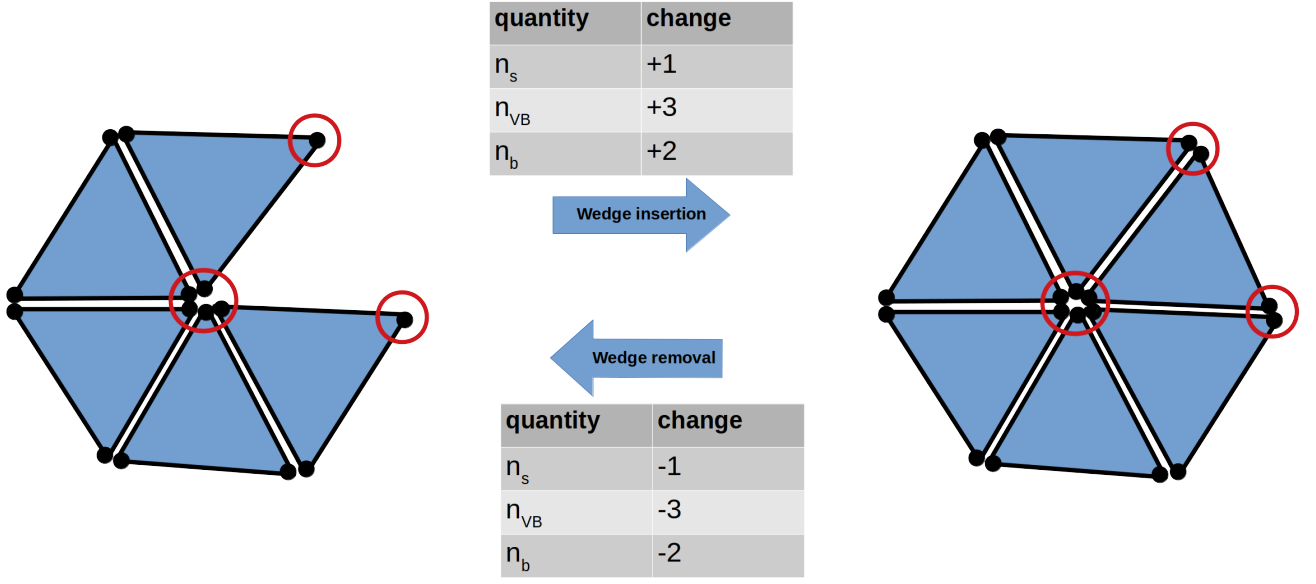

FIG. 16: Wedge insertion and removal.

Using Eqs. (23) and (25), the acceptance probability for fusion moves is

$$p_{\text{acc}}(i \rightarrow j) = \min \left[ 1, \frac{v_a}{v_{\text{fuse}}} \exp(-\Delta E_{i \rightarrow j}/k_B T) \right] \quad (24)$$

where  $v_{\text{fuse}} = (4\pi/3)(l_{\text{fuse}}/2)^3$  is the volume of a sphere with diameter  $l_{\text{fuse}}$ , and  $\Delta E_{i \rightarrow j}$  is the energy change due to the fusion, including changes in bending, stretching, and binding energies. A fusion move increases the number of edge bonds and vertex bonds by one,  $n_b \rightarrow n_b + 1$  and  $n_{VB} \rightarrow n_{VB} + 1$ ; the factor of  $v_a$  appears in Eq. (24) to account for the latter.

## 2. Wedge fission

Wedge fission, in which a wedge is opened, is the reverse of the wedge fusion move. Fissionable edges are those edges that can be split along their boundary vertex to obtain a wedge. Denoting the number of such edges as  $n_f$ , the probability of attempting a wedge fission move during an MC step is  $n_f k_{\text{wf}} \tau$ . If a fission move is attempted, then an edge is selected randomly from the  $n_f$  fissionable edges. The position of one of the new vertices is selected randomly within the sphere of volume  $v_{\text{fuse}}$  centered at the original position of the merged vertices, and the other new vertex is placed in the opposite direction from the original position, at the same distance. Thus, the attempt generation probability is

$$\alpha(j \rightarrow i) = n_f k_{\text{wf}} \tau \times \frac{1}{n_f (v_{\text{fuse}}/d\vec{x})} \quad (25)$$

and the acceptance probability is

$$p_{\text{acc}}(j \rightarrow i) = \min \left[ 1, \frac{v_{\text{fuse}}}{v_a} \exp(-\Delta E_{j \rightarrow i}/k_B T) \right] \quad (26)$$

We verify that detailed balance holds between wedge fusion and fission as follows. There are two cases to consider:

1.  $(v_{\text{fuse}}/v_a) \exp(-\Delta E_{j \rightarrow i}/k_B T) < 1 \Leftrightarrow (v_a/v_{\text{fuse}}) \exp(-\Delta E_{i \rightarrow j}/k_B T) > 1$

In this case,  $p_{\text{acc}}(i \rightarrow j) = 1$  and  $p_{\text{acc}}(j \rightarrow i) = (v_{\text{fuse}}/v_a) \exp(-\Delta E_{j \rightarrow i}/k_B T)$ . Then

$$P_i \times \alpha(i \rightarrow j) \times p_{\text{acc}}(i \rightarrow j) = \frac{1}{Z_\Omega} v_a^{n_{VB,i}} \exp[-(E_i - \mu_{s,i})/k_B T] \frac{1}{\lambda^{9n_{s,i}}} \times d^{n_{v,i}} \vec{x} \times k_{\text{wf}} \tau \quad (27)$$

and

$$P_j \times \alpha(j \rightarrow i) \times p_{\text{acc}}(j \rightarrow i) = \frac{1}{Z_\Omega} v_a^{n_{\text{VB},j}} \exp[-(E_j - \mu n_{s,j})/k_B T] \frac{1}{\lambda^{9n_{s,j}}} \times d^{n_{v,j}} \vec{x} \quad (28)$$

$$\times k_{\text{wf}} \tau d\vec{x} / v_{\text{fuse}} \times (v_{\text{fuse}}/v_a) \exp(-\Delta E_{j \rightarrow i}/k_B T) \quad (29)$$

Using:  $\Delta E_{j \rightarrow i} = E_i - E_j$ ,  $n_{s,i} = n_{s,j}$  (because the move leaves the subunit number unchanged),  $n_{\text{VB},i} = n_{\text{VB},j} - 1$  (one vertex bond is broken upon fission) and  $n_{v,i} = n_{v,j} + 1$  (an extra vertex is being born upon fission), we see that the two are equal and detailed balance holds.

2.  $(v_{\text{fuse}}/v_a) \exp(-\Delta E_{j \rightarrow i}/k_B T) > 1 \Leftrightarrow (v_a/v_{\text{fuse}}) \exp(-\Delta E_{i \rightarrow j}/k_B T) < 1$

In this case,  $p_{\text{acc}}(i \rightarrow j) = (v_a/v_{\text{fuse}}) \exp(-\Delta E_{i \rightarrow j}/k_B T)$  and  $p_{\text{acc}}(j \rightarrow i) = 1$ . Then

$$P_i \times \alpha(i \rightarrow j) \times p_{\text{acc}}(i \rightarrow j) = \frac{1}{Z_\Omega} v_a^{n_{\text{VB},i}} \exp[-(E_i - \mu n_{s,i})/k_B T] \frac{1}{\lambda^{9n_{s,i}}} \times d^{n_{v,i}} \vec{x} \times k_{\text{wf}} \tau \quad (30)$$

$$\times (v_a/v_{\text{fuse}}) \exp(-\Delta E_{i \rightarrow j}/k_B T) \quad (31)$$

and

$$P_j \times \alpha(j \rightarrow i) \times p_{\text{acc}}(j \rightarrow i) = \frac{1}{Z_\Omega} v_a^{n_{\text{VB},j}} \exp[-(E_j - \mu n_{s,j})/k_B T] \frac{1}{\lambda^{9n_{s,j}}} \times d^{n_{v,j}} \vec{x} \quad (32)$$

$$\times k_{\text{wf}} \tau d\vec{x} / v_{\text{fuse}} \quad (33)$$

Using again  $\Delta E_{j \rightarrow i} = E_i - E_j$ ,  $n_{s,i} = n_{s,j}$ ,  $n_{\text{VB},i} = n_{\text{VB},j} - 1$  and  $n_{v,i} = n_{v,j} + 1$ , detailed balance holds.

Note that detailed balance is satisfied regardless of the values of  $k_{\text{wf}} \tau$  or  $v_{\text{fuse}}$ , but as with all of the move frequencies these parameters can be optimized during burn-in to accelerate convergence to the equilibrium distribution  $P(i)$ . In our simulations, we find that the optimal value of  $v_{\text{fuse}}$  is on the order of the optimal value of  $d_{\text{max}}$  for analogous reasons: if  $v_{\text{fuse}}$  is too small there will be very few vertex pairs identified as fusable, so  $n_w$  will be low. If  $v_{\text{fuse}}$  is too large, there will be many fusion candidates but most fusion attempts will be rejected due to the large elastic energy change necessary for the merging deformation.

Most importantly, we note the constraint on the parameters  $k_{\text{wf}} \tau$  to ensure that generation probabilities do not become larger than unity. Because each attempt is generated as a three step process, using three probabilities, one has to ensure that all those probabilities are less than 1. Specifically,

$$n_w k_{\text{wf}} \tau < 1 \quad (34)$$

$$n_f k_{\text{wf}} \tau < 1. \quad (35)$$

## E. Crack fusion / fission

### 1. Crack fusion

Crack fusion closes a crack within the structure; i.e., two adjacent pairs of edges are merged (Fig. 18). Cracks are identified as 4-edge-length holes inside the structure. If the vertices of the hole are labeled A, B, C, D then the polygon ABCD forms a closed loop (see Fig. 18). The crack can be closed by either merging vertices A and C (and correspondingly edges CD to DA and AB to BC) or by merging vertices B and D (and correspondingly edges AD to AB and CD to CB). Each 4-edge-length loop thus defines two potential fusable cracks. However, an additional condition for a crack to be fusable is that its merging vertices must be within a distance  $l_{\text{fuse}}$  (A and C or D and B in this example). In this work, we have set the crack fusion volume to be the same as that for wedge fusion to reduce the number of parameters, but it is not necessary that they be the same and the acceptance probability is

$$p_{\text{acc}}(i \rightarrow j) = \min \left[ 1, \frac{v_a}{v_{\text{fuse}}} \exp(-\Delta E_{i \rightarrow j}/k_B T) \right] \quad (36)$$

There are two edge bonds and one vertex bond formed during a crack fusion.

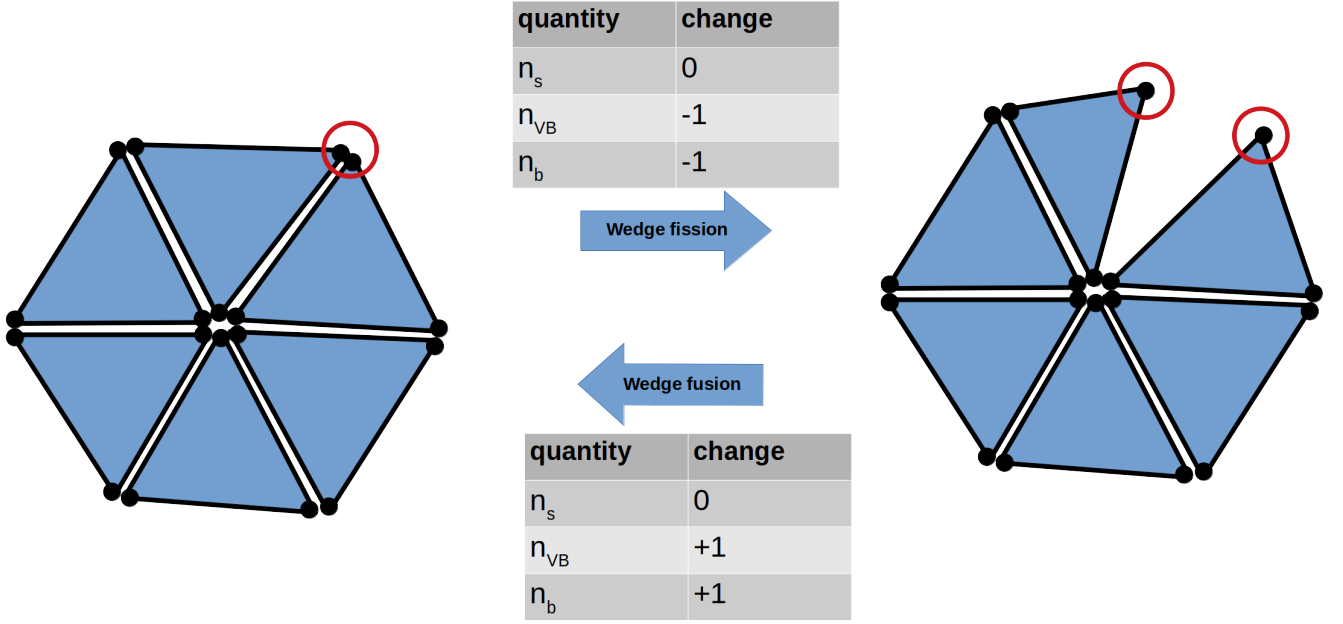

FIG. 17: Wedge fusion and fission.

## 2. Crack fission

The reverse move for crack fusion is crack fission. With the number of potential cracks as  $n_{cf}$ :

$$\alpha(j \rightarrow i) = n_{cf} k_{cf} \tau \times \frac{1}{n_{cf} (v_{fuse}/d\vec{x})} \quad (37)$$

$$p_{acc}(j \rightarrow i) = \min \left[ 1, \frac{v_{fuse}}{v_a} \exp(-\Delta E_{j \rightarrow i}/k_B T) \right] \quad (38)$$

As for the case of wedge fusion/fission, the crack fusion attempt frequency parameter  $k_{cf}$  is constrained by the conditions maintaining probabilities smaller than unity:

$$n_c k_{cf} \tau < 1 \quad (39)$$

$$n_{cf} k_{cf} \tau < 1 \quad (40)$$

$$(41)$$

## F. Edge fusion / fission

### 1. Edge fusion

During this move two non-neighbor edges are fused (Fig. 19). Fusable edges are non-neighboring edge pairs whose corresponding vertices are within a separation distance  $l_{fuse}$ . Since edges are directed, they can only fuse such that, after fusion, they point in the opposite direction. Assuming the edges to be fused are  $A \rightarrow B$  and  $C \rightarrow D$  (see Fig. 19), vertex  $A$  will merge into vertex  $D$  and vertex  $B$  will merge into vertex  $C$ . Edges are counted as fusable if  $A$  is within a distance  $l_{fuse}$  to  $D$  and  $B$  is also within a distance  $l_{fuse}$  to  $C$ . The attempt probability is analogous to that for wedge and crack fusion/fission,

$$\alpha(i \rightarrow j) = n_e k_{ef} \tau \times \frac{1}{n_e} \quad (42)$$

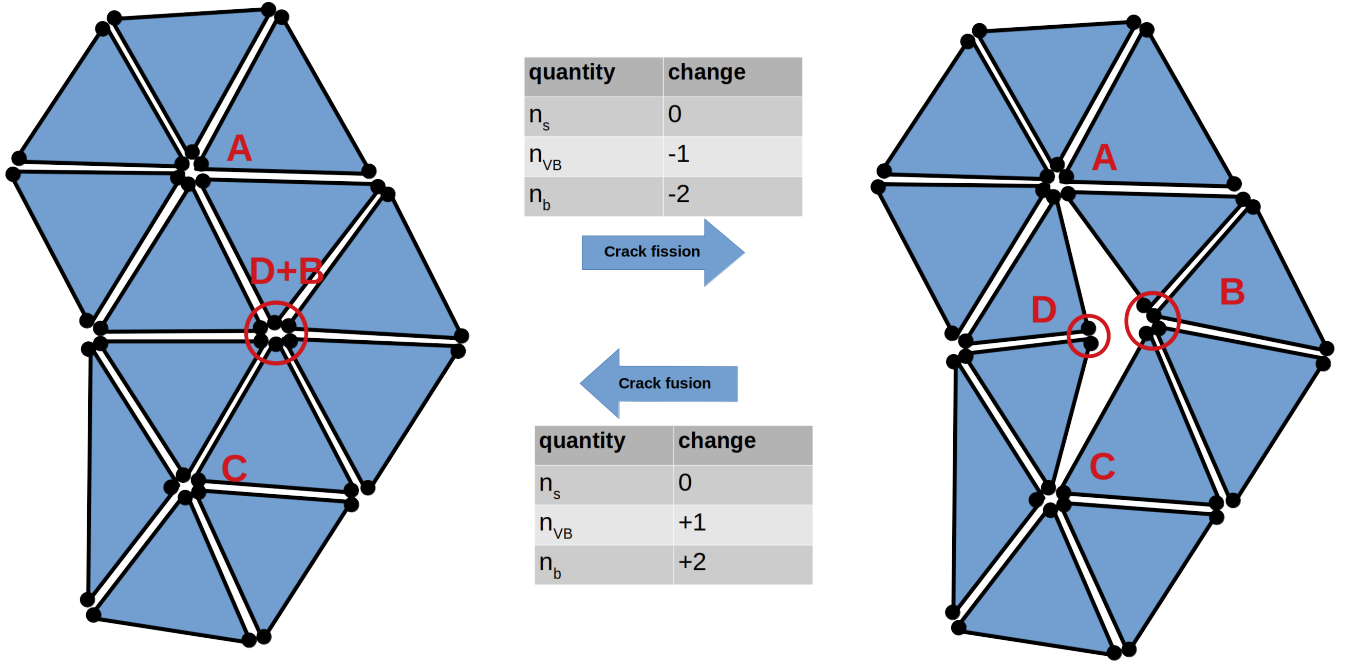

FIG. 18: Crack fusion and fission.

with  $n_e$  the number of fusable edges and  $k_{ef}$  the edge fusion frequency parameter. The acceptance probability is

$$p_{acc}(i \rightarrow j) = \min \left[ 1, \left( \frac{v_a}{v_{fuse}} \right)^2 \exp(-\Delta E_{i \rightarrow j} / k_B T) \right] \quad (43)$$

During edge fusion, one edge bond and two vertex bonds are created.

## 2. Edge fission

Edge fission is the reverse move of edge fusion.  $n_{ef}$  is the number of breakable edges, that is, those edges that have both vertices on the boundary and which would not result in breaking the structure apart.

$$\alpha(j \rightarrow i) = n_{ef} k_{ef} \tau \times \frac{1}{n_{ef} (v_{fuse} / d\vec{x})^2} \quad (44)$$

The factor  $1/(v_{fuse})^2$  arises because we must select a random position for each pair of vertices, independently. The acceptance probability is then

$$p_{acc}(j \rightarrow i) = \min \left[ 1, \left( \frac{v_{fuse}}{v_a} \right)^2 \exp(-\Delta E_{j \rightarrow i} / k_B T) \right]. \quad (45)$$

To maintain probabilities within unity, the edge fusion frequency parameter  $k_{ef}$  is constrained by

$$n_e k_{ef} \tau < 1 \quad (46)$$

$$n_{ef} k_{ef} \tau < 1. \quad (47)$$

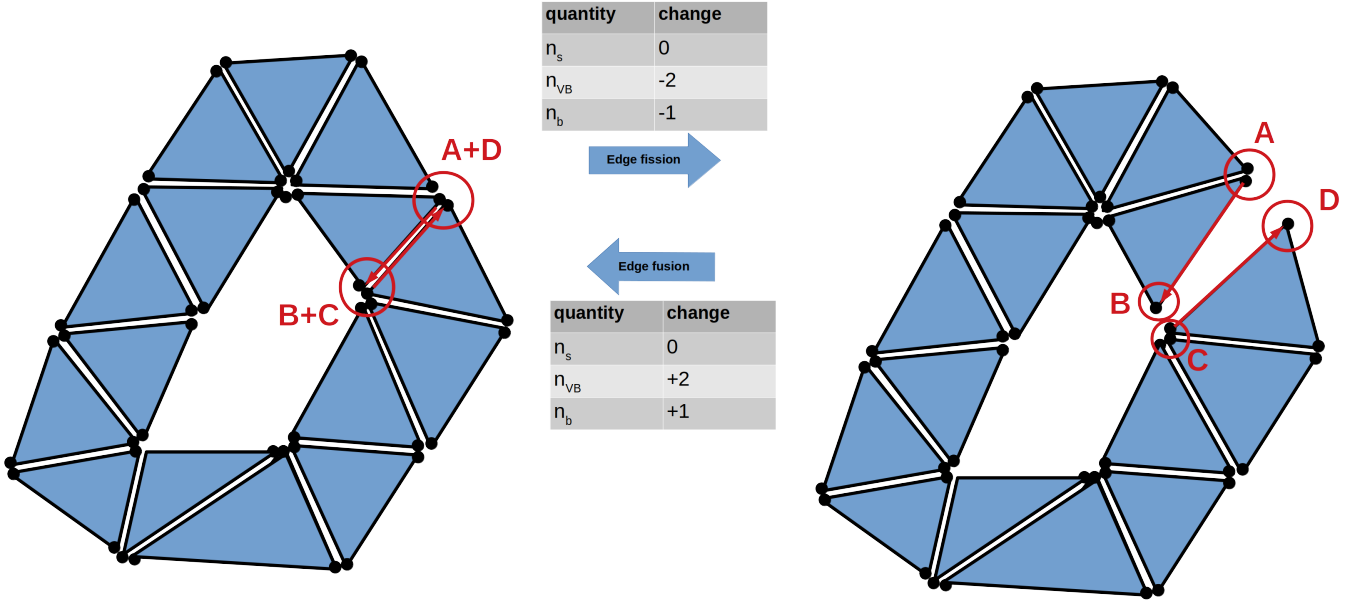

FIG. 19: Edge fusion and fission.

- [2] T. Dotera, H. Tanaka, and Y. Takahashi, *Structural Chemistry* **28**, 105 (2017), ISSN 1040-0400, 1572-9001, URL <http://link.springer.com/10.1007/s11224-016-0833-7>.
- [3] T. E. Videbaek, H. Fang, D. Hayakawa, B. Tyukodi, M. F. Hagan, and W. B. Rogers, *Journal of Physics: Condensed Matter* **34**, 134003 (2022), URL <https://dx.doi.org/10.1088/1361-648X/ac47dd>.
- [4] B. Tyukodi, F. Mohajerani, D. M. Hall, G. M. Grason, and M. F. Hagan, *ACS Nano* (2022), ISSN 1936-0851, 2109.01174.
- [5] H. Fang, B. Tyukodi, W. B. Rogers, and M. F. Hagan, *Soft Matter* **18**, 6716 (2022), ISSN 17446848, 2205.11598.
- [6] C. Sigl, E. M. Willne, W. Engelen, J. A. Kretzmann, K. Sachenbacher, A. Liedl, F. Kolbe, F. Wilsch, S. A. Aghvami, U. Protzer, et al., *Nature Materials* **20**, 1281–1289 (2021).
- [7] G. M. Rotskoff and P. L. Geissler, *Proceedings of the National Academy of Sciences of the United States of America* **115**, 6341 (2018), ISSN 10916490, 1709.00321.
- [8] M. Botsch, S. Steinberg, S. Bischoff, and L. Kobbelt, in *OpenSG Symposium* (2002).
- [9] D. Frenkel and B. Smit, *Understanding molecular simulation: From algorithms to applications* (1996).
